# Supplementary material for: IM360: Large-scale Indoor Mapping with 360 Cameras
Source: arXiv:2502.12545 source file (2025-09-28)
Supplement: Supplementary file 1 [file render_comparison_supp1.pdf]

2t7WUuJek07

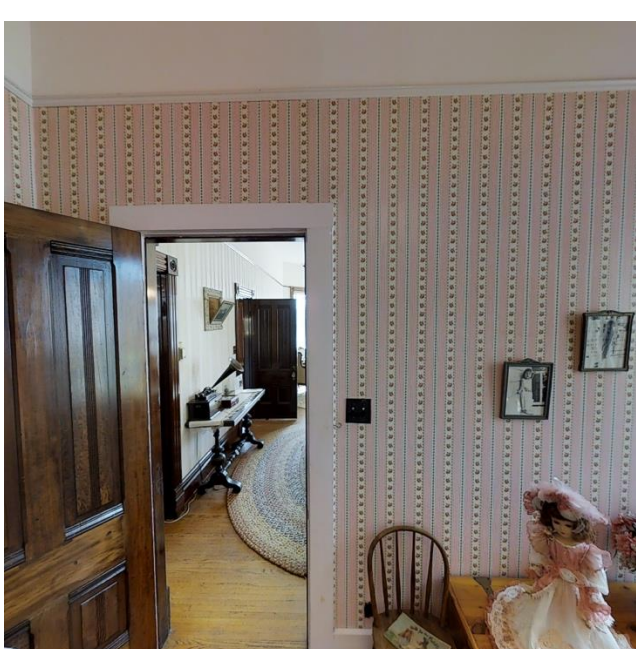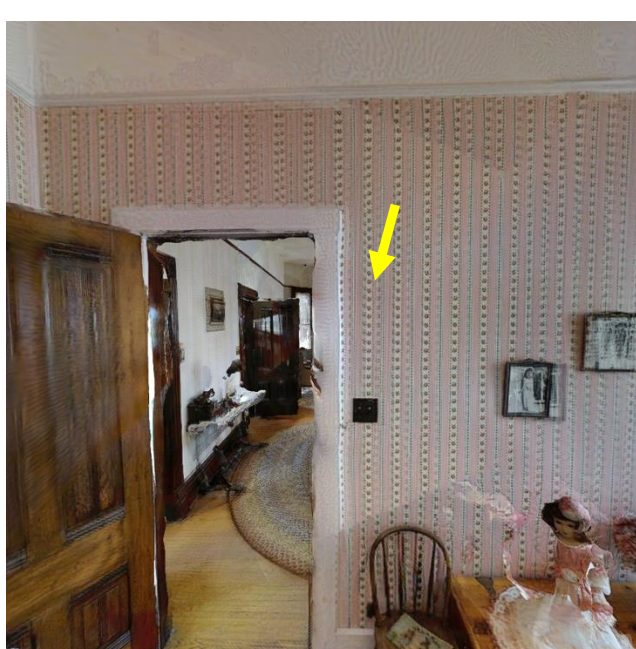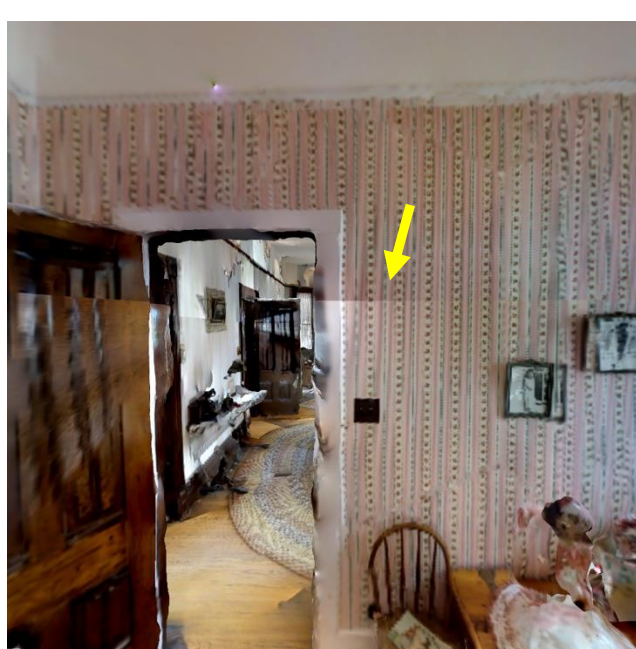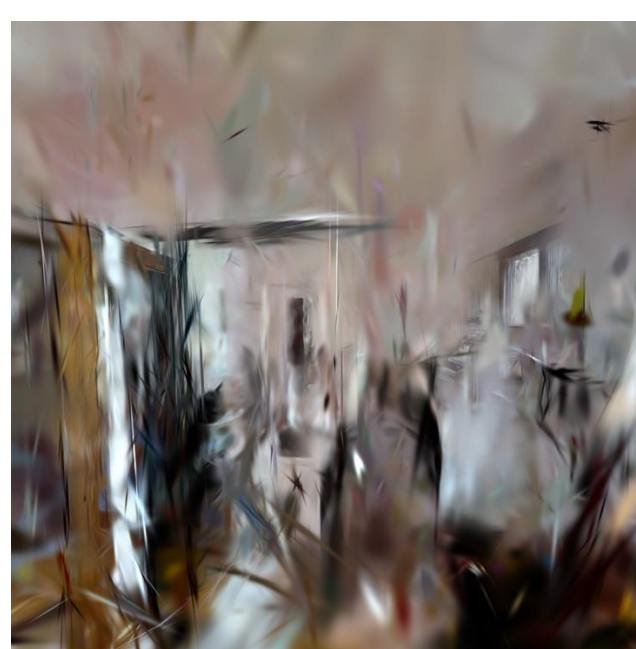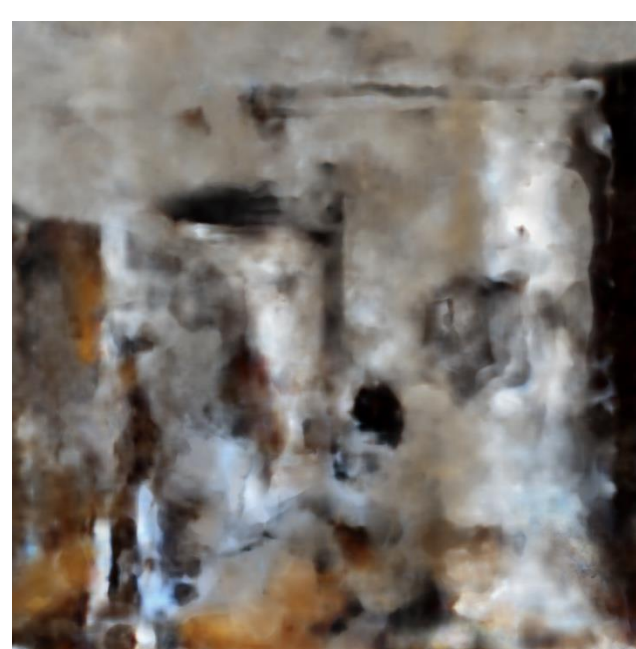

YVUC4YcDtcY

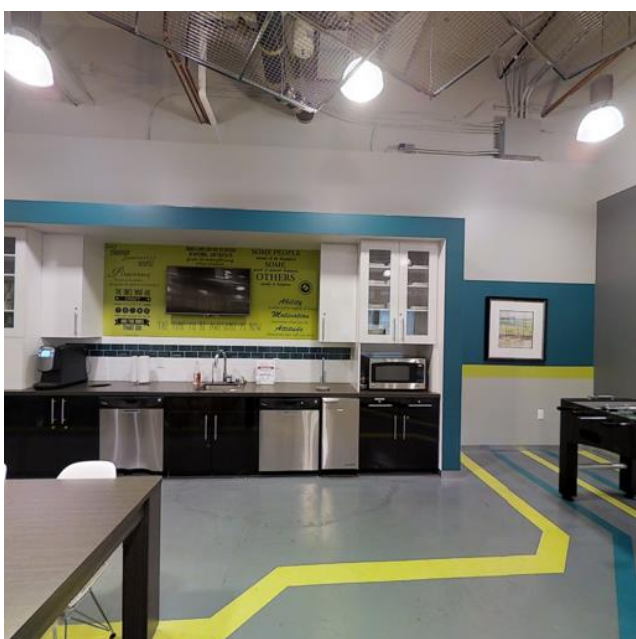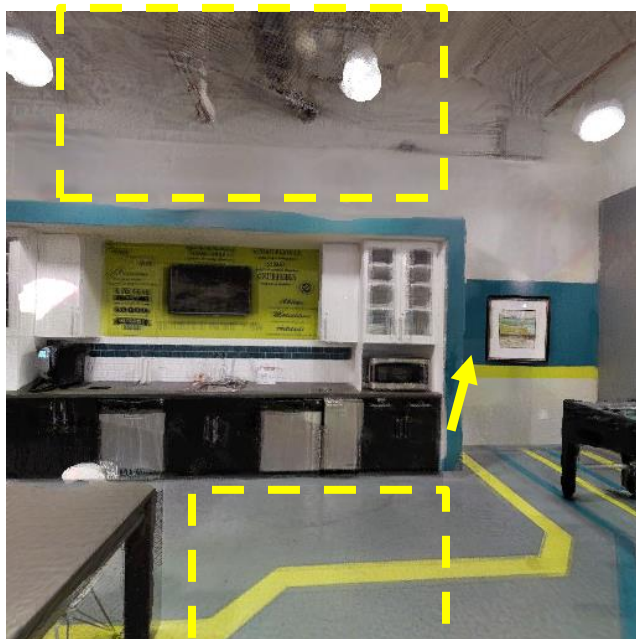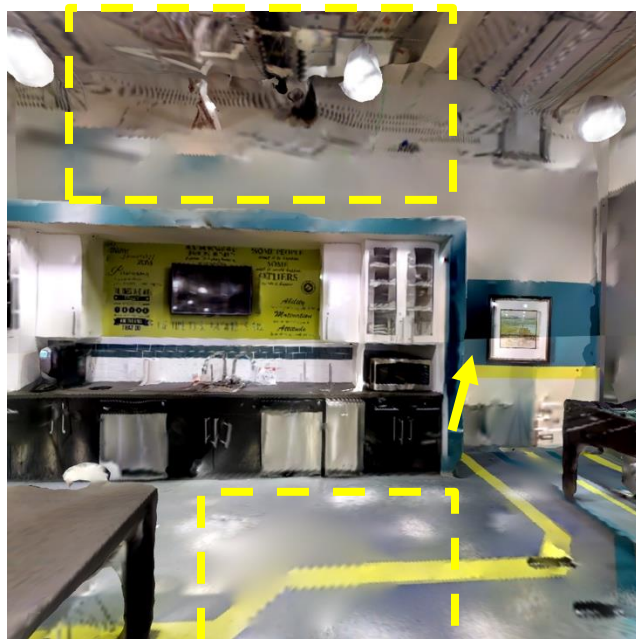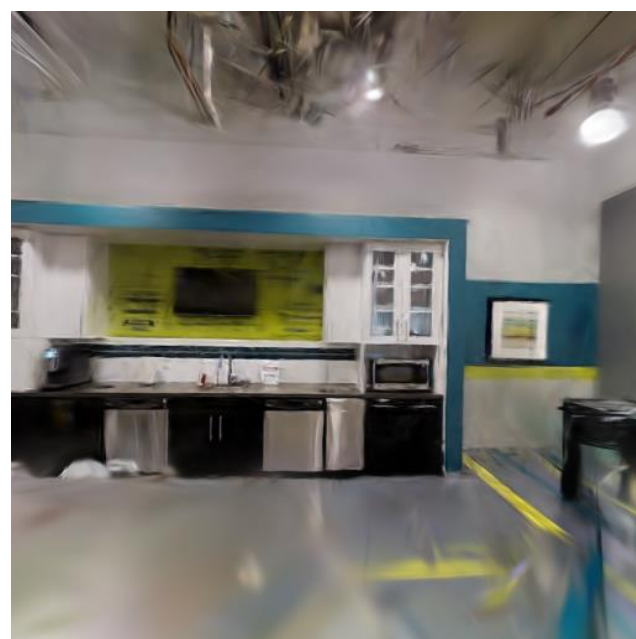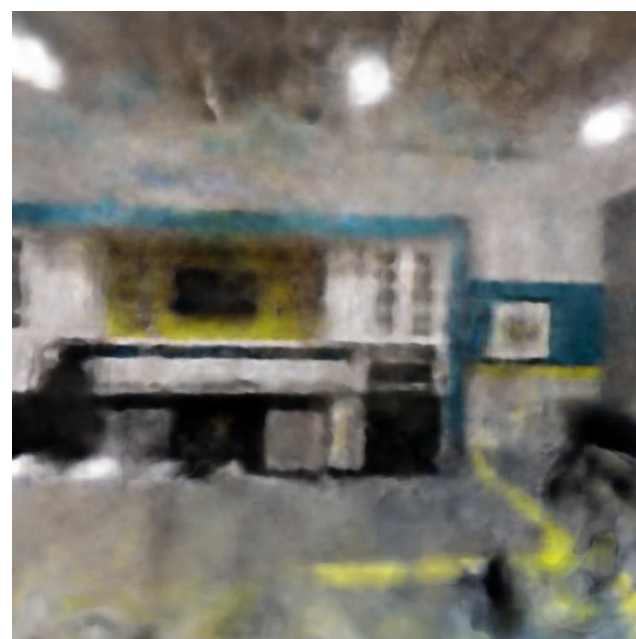

pLe4wQe7qrG

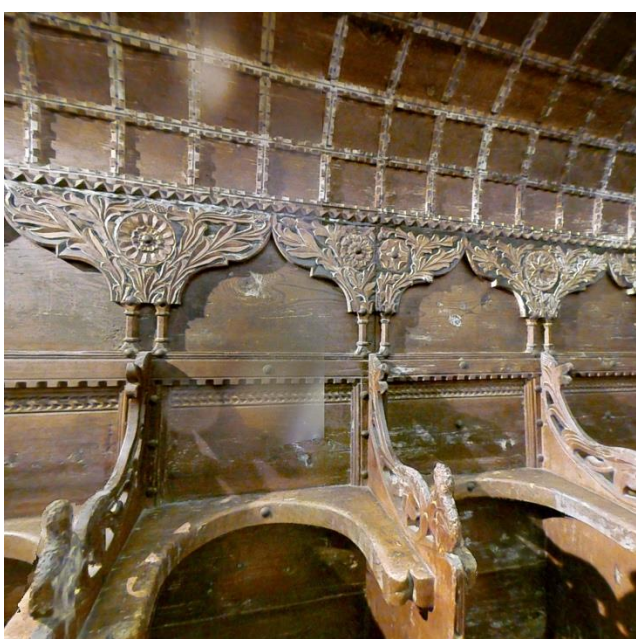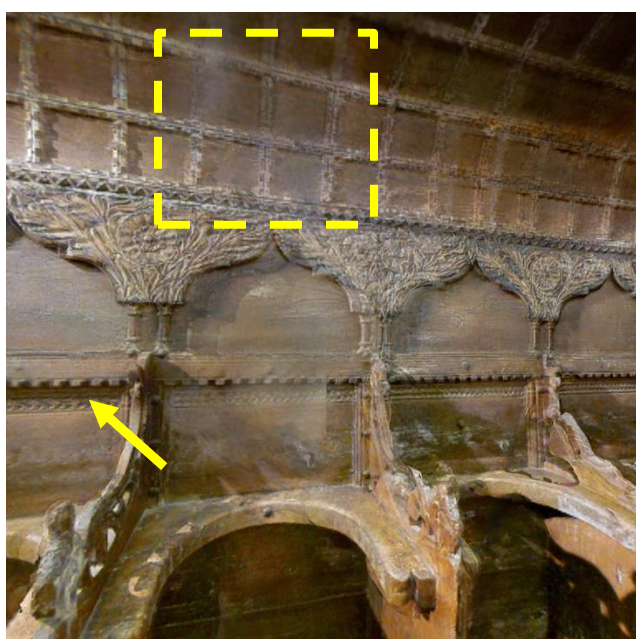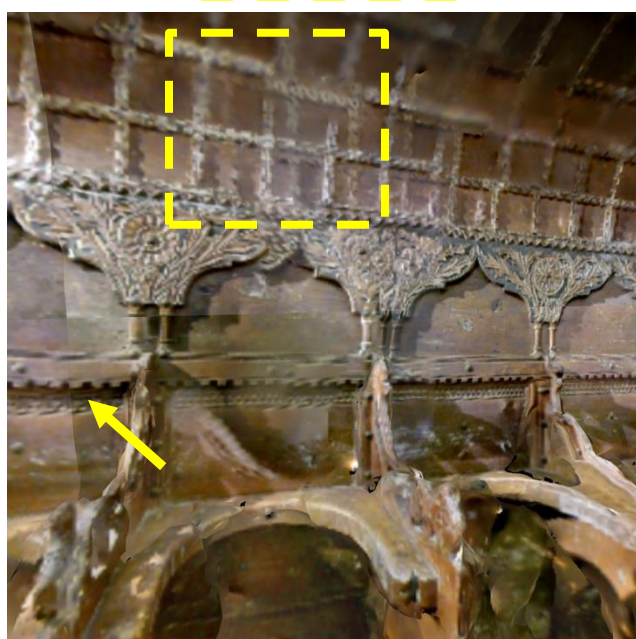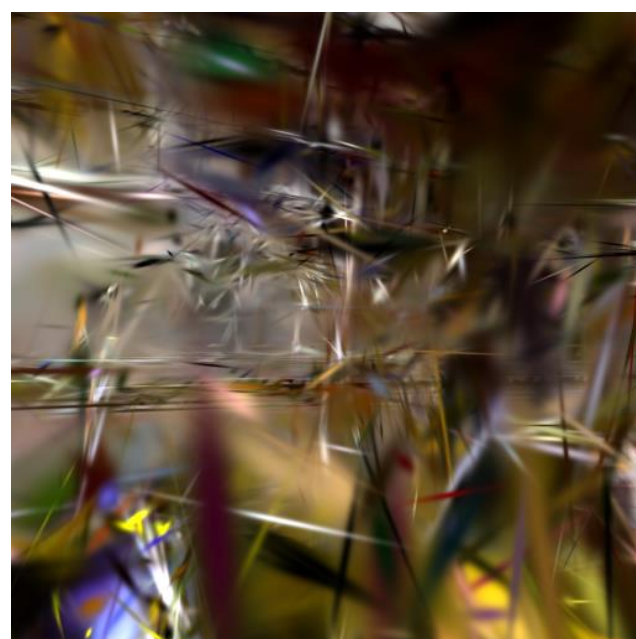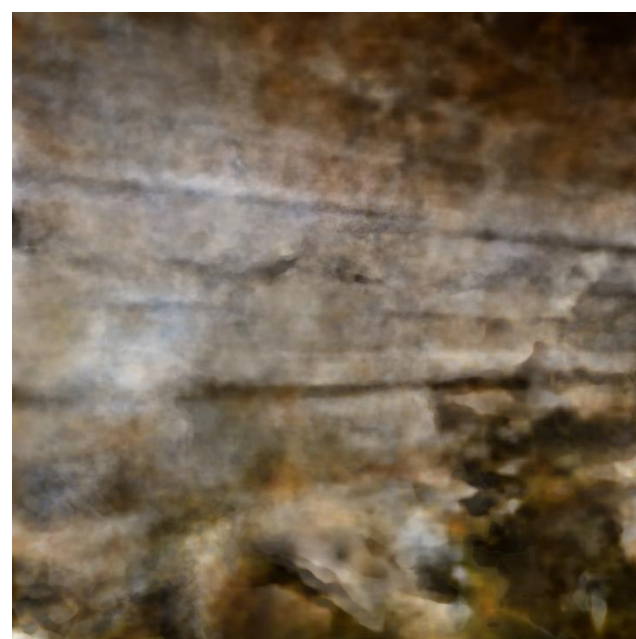

RPMz2sHmrrY

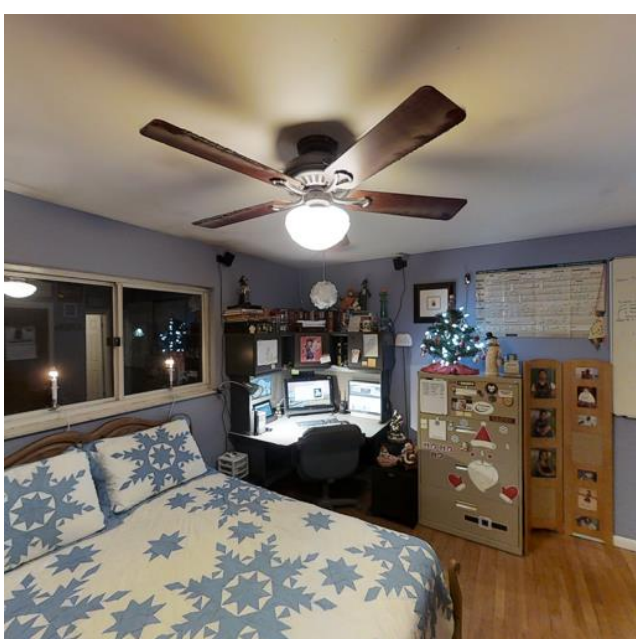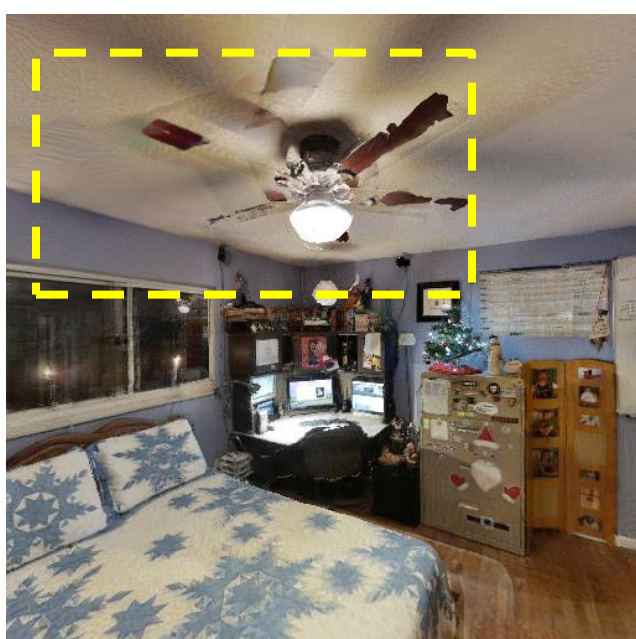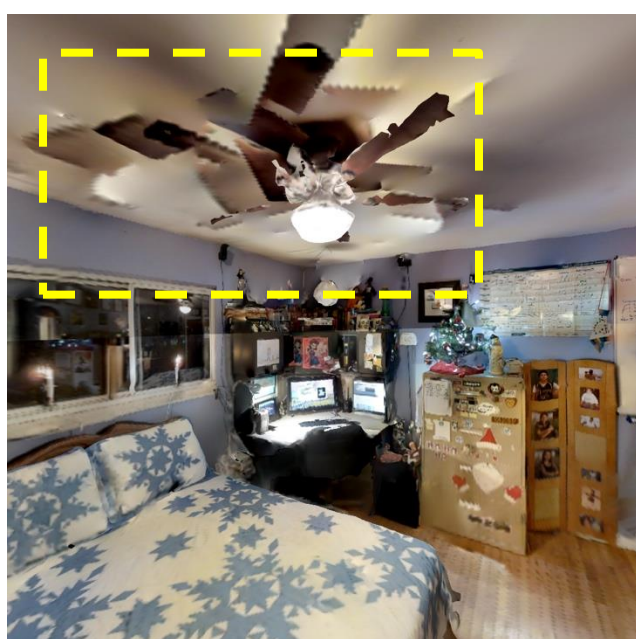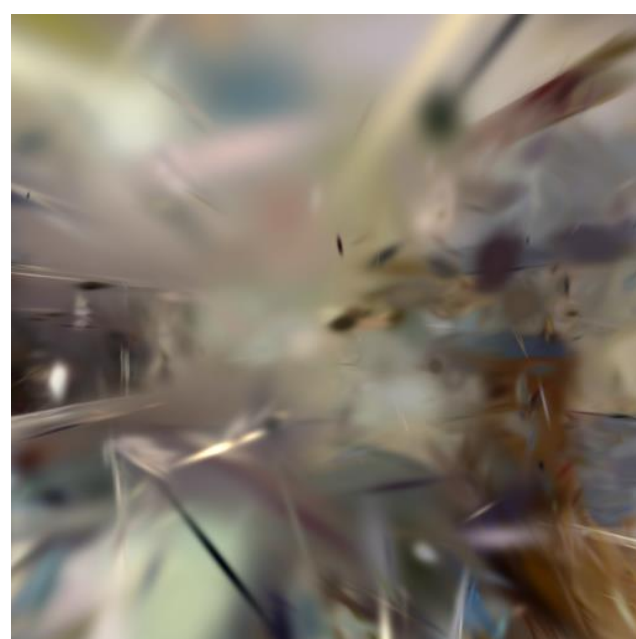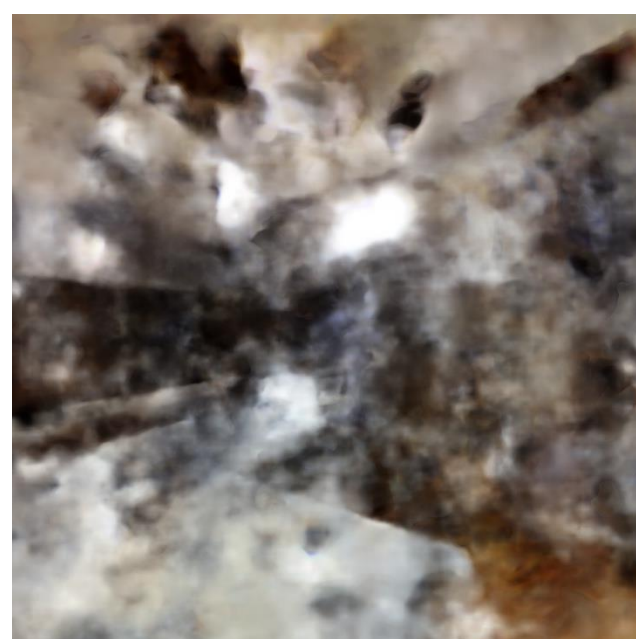

8194nk7LbLH

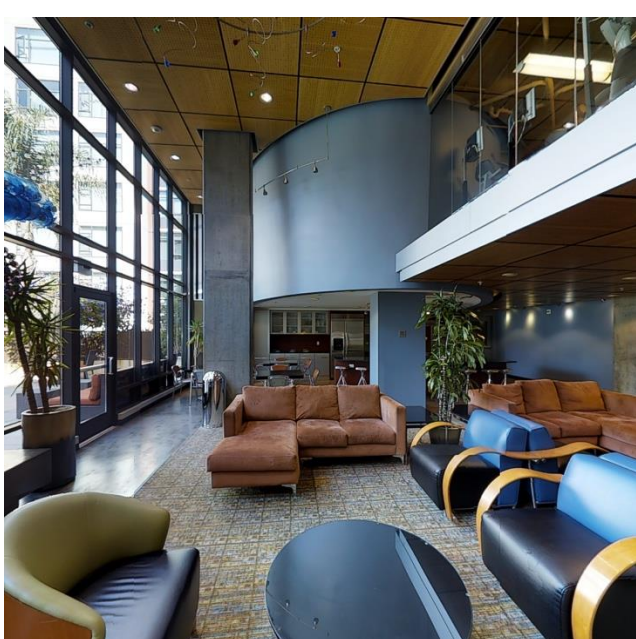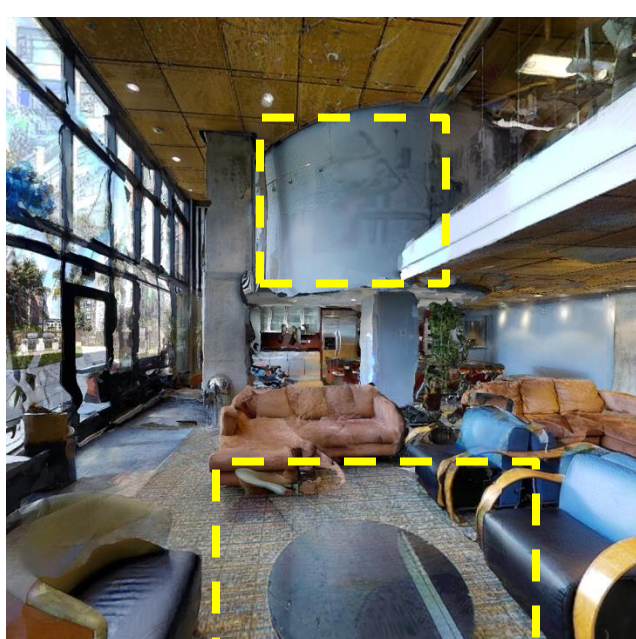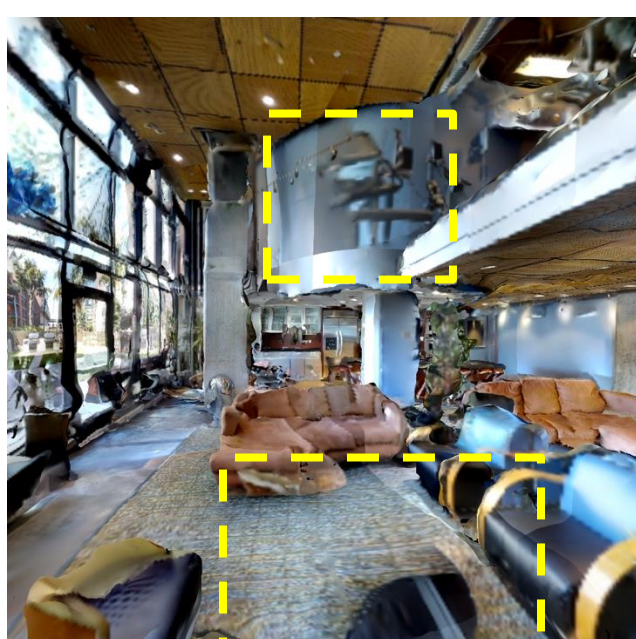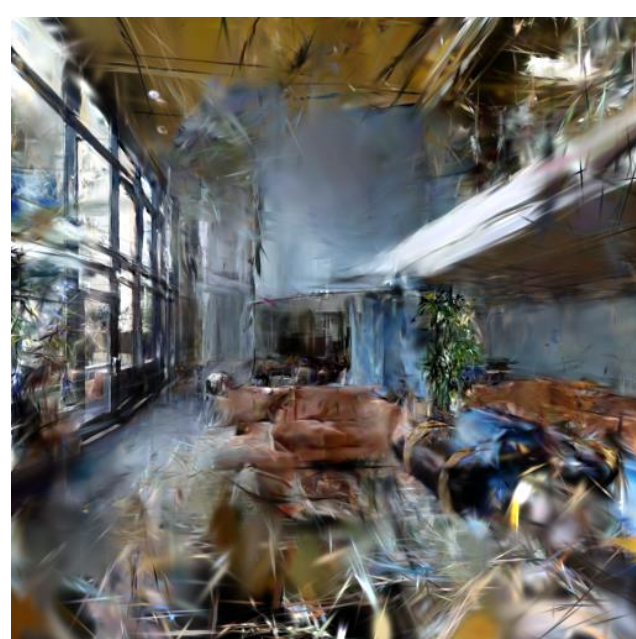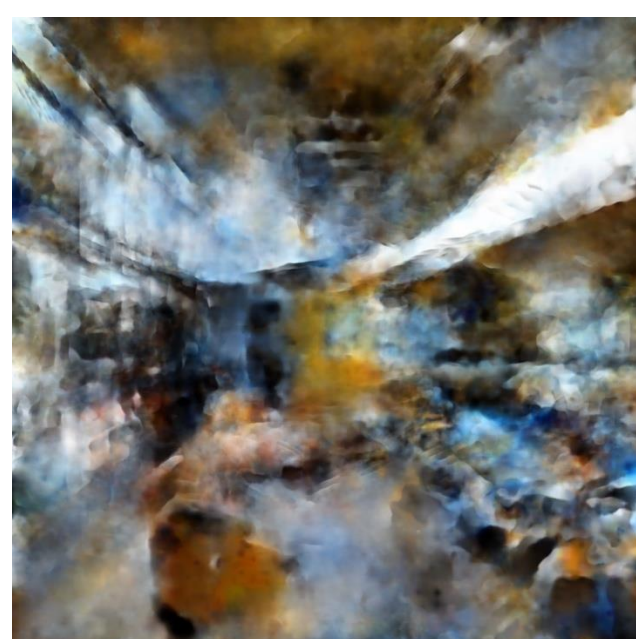

zsNo4HB9uLZ

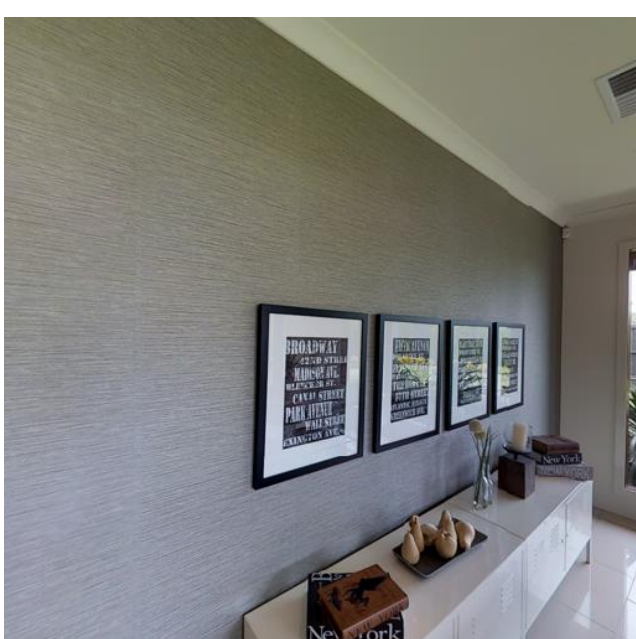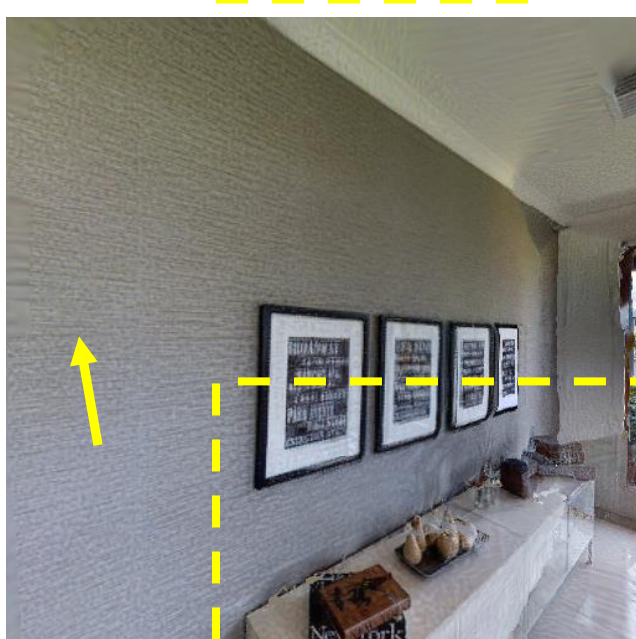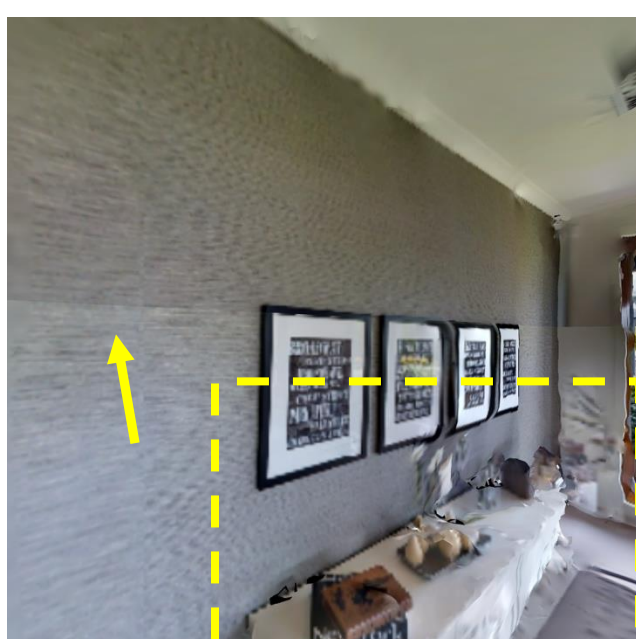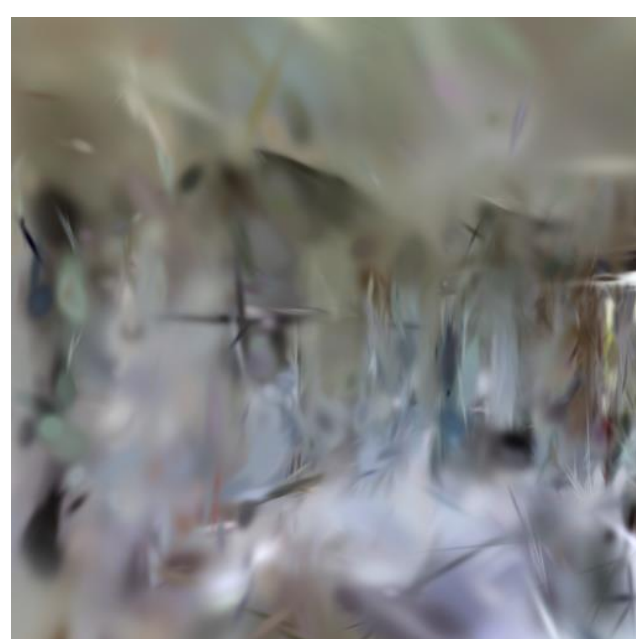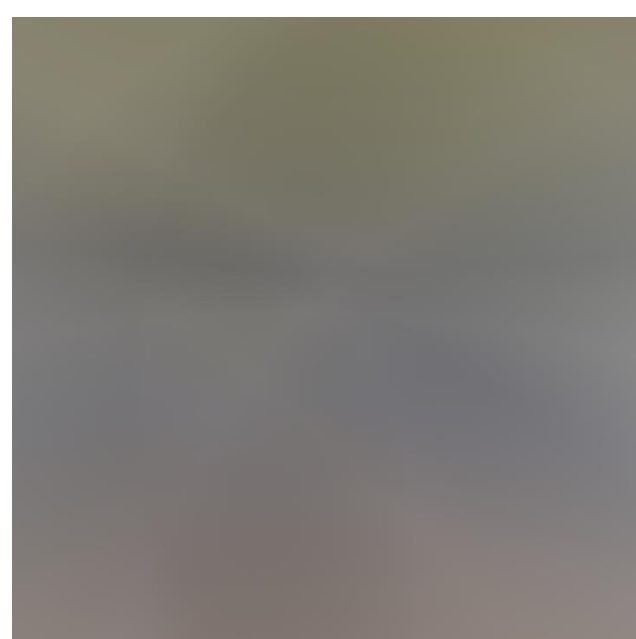

Scene

(a) Ours

(b) TexRecon

(c) SparseGS

(d) ZipNeRF

2t7WUuJek07

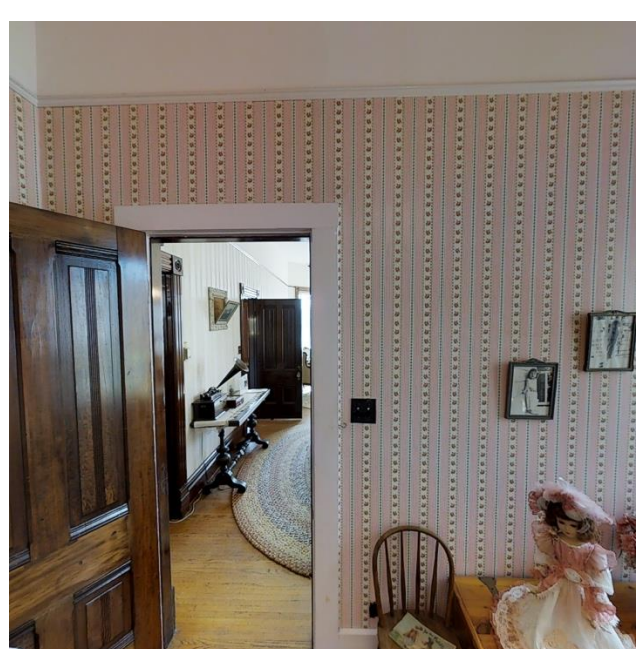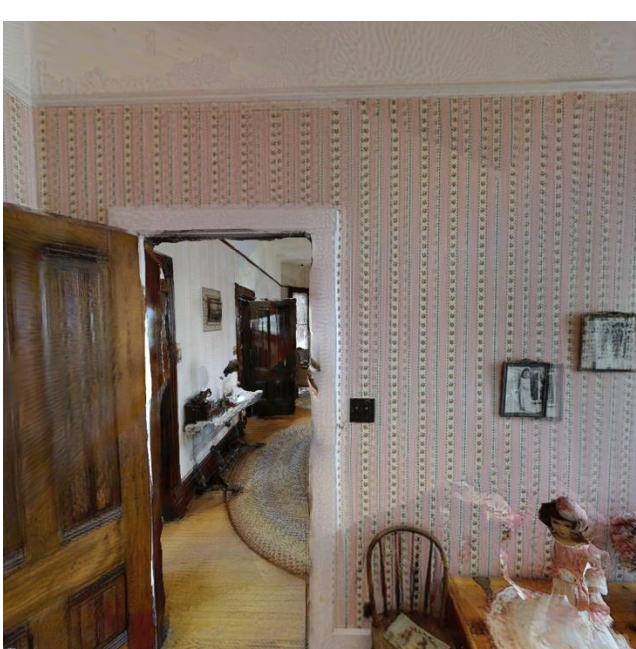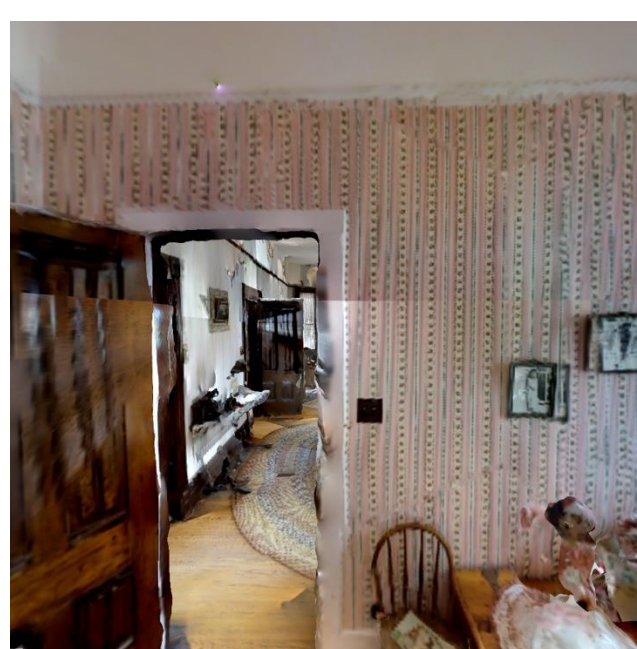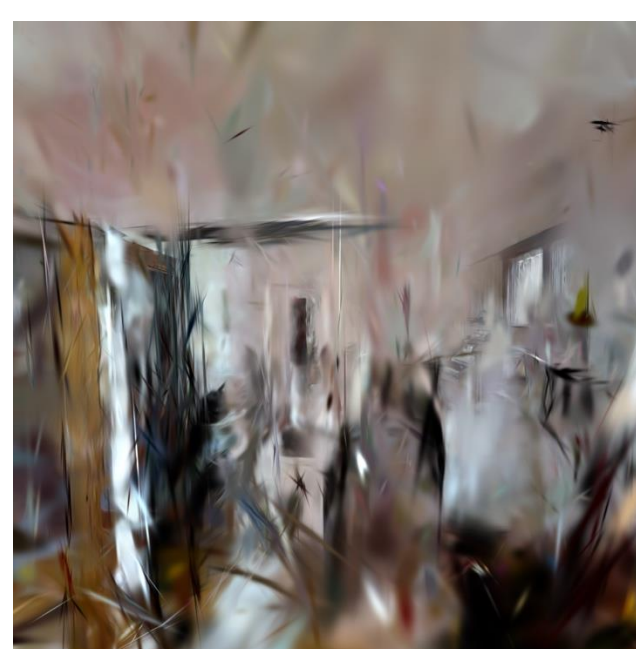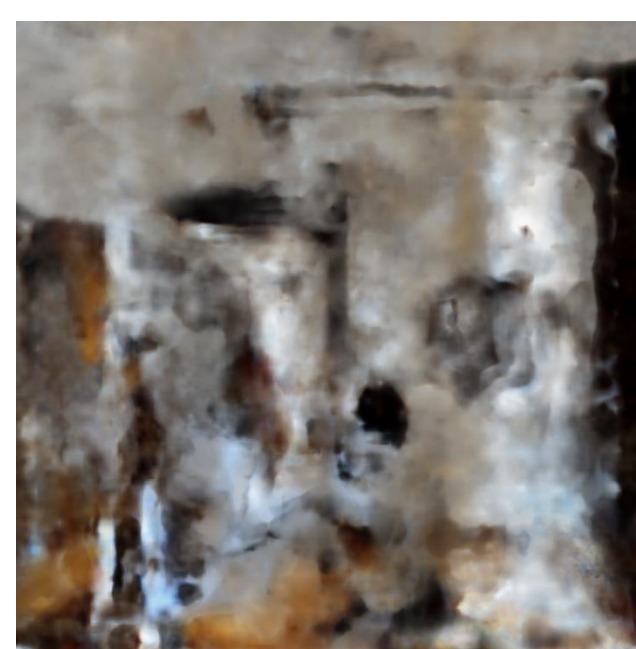

YVUC4YcDtcY

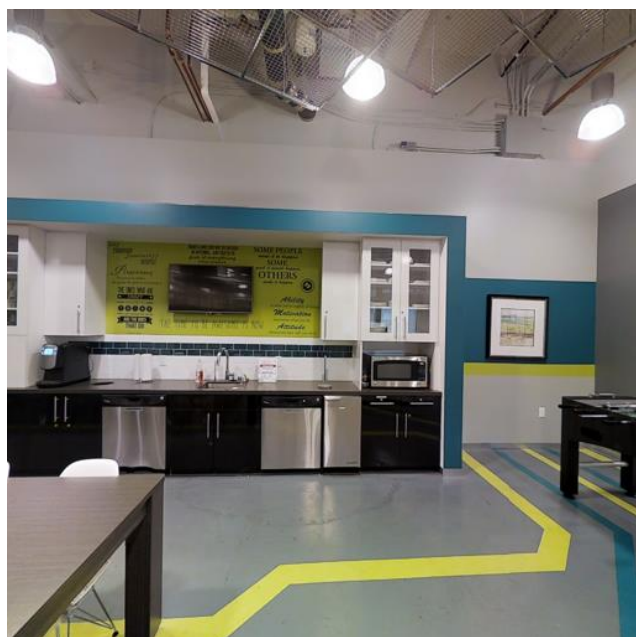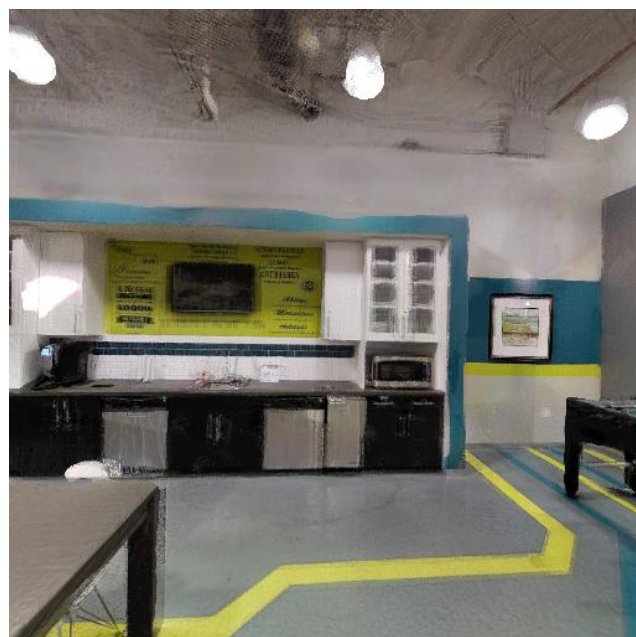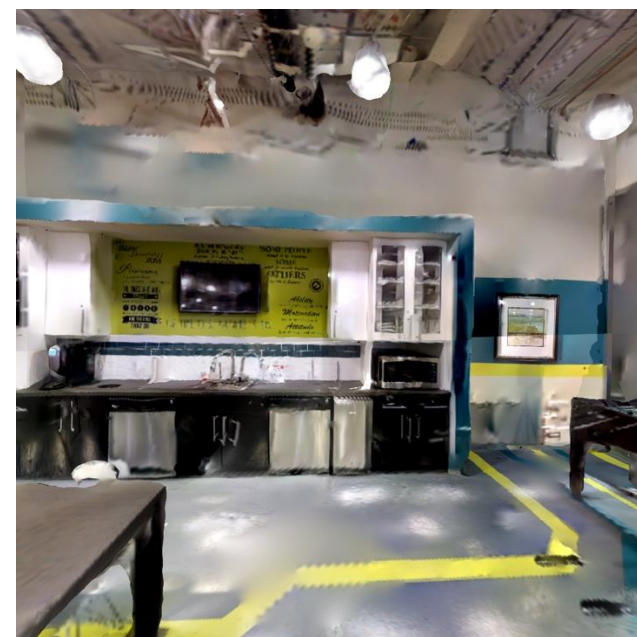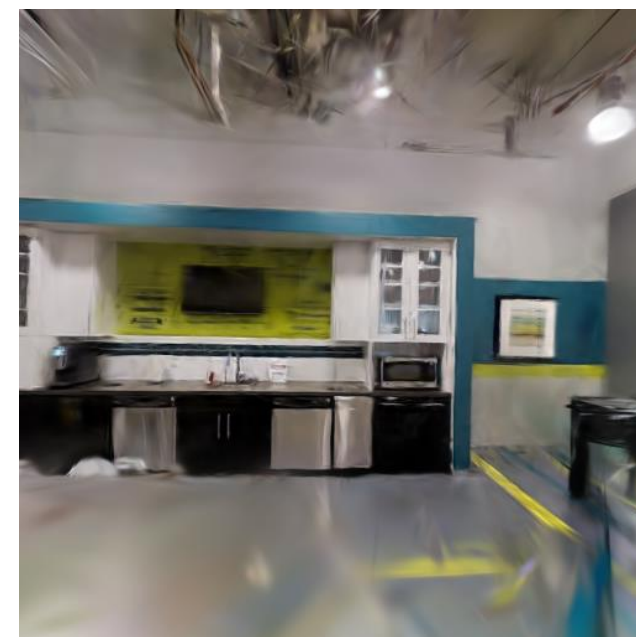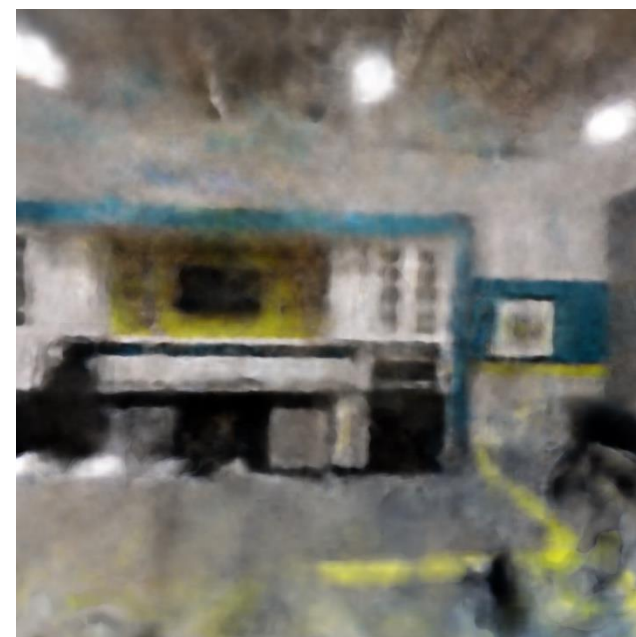

pLe4wQe7qrG

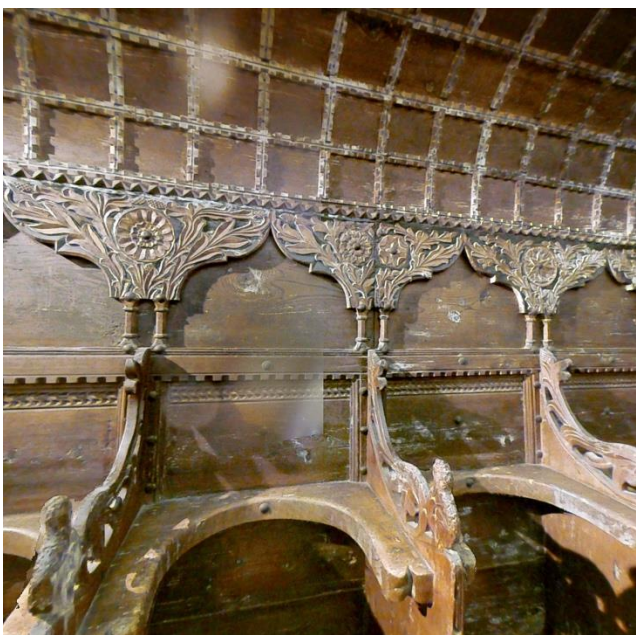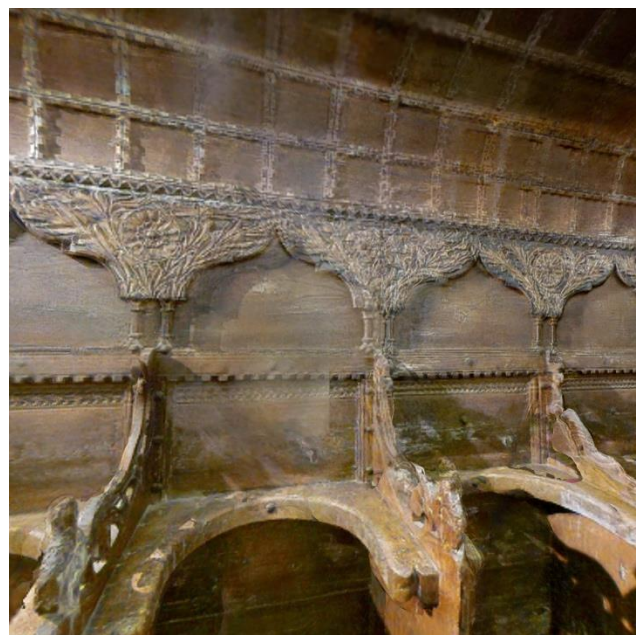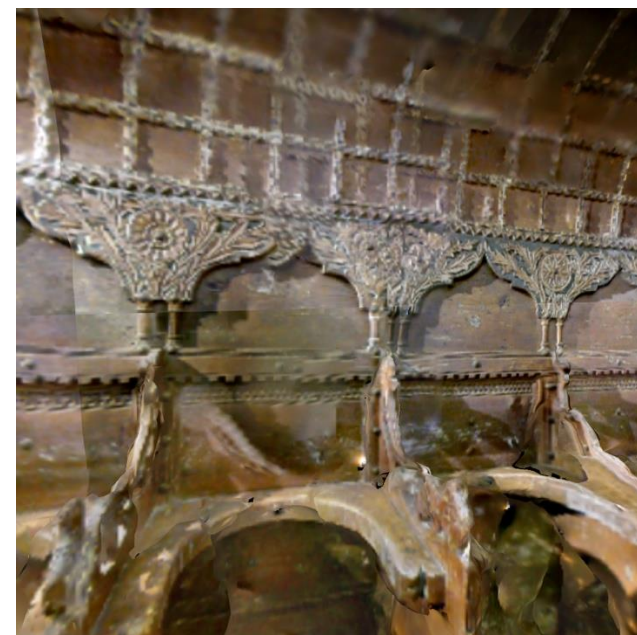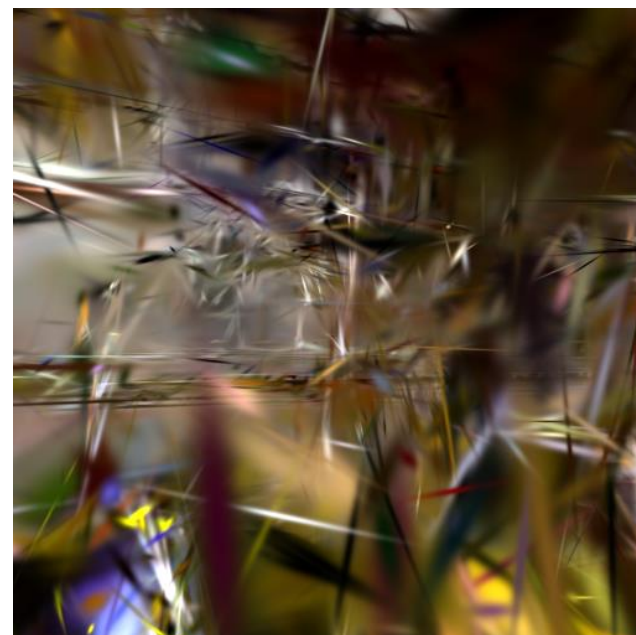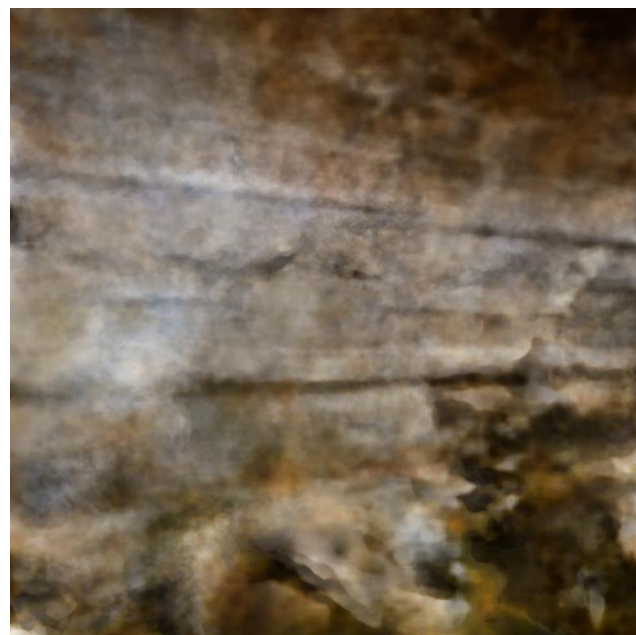

RPmz2sHmrrY

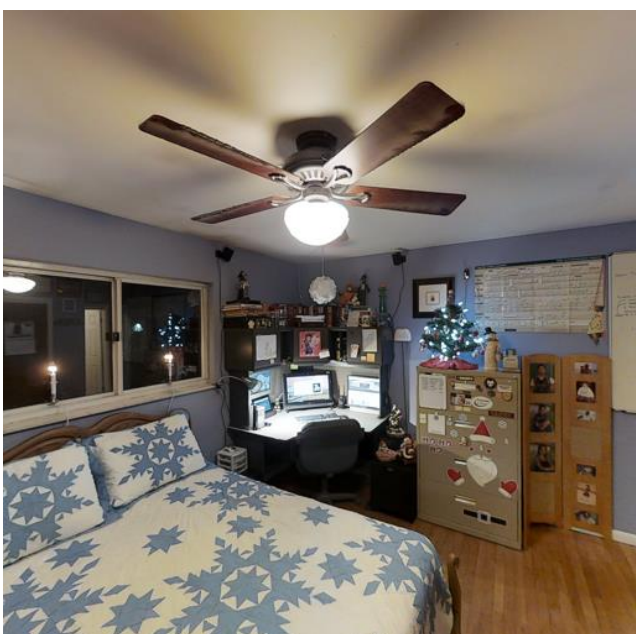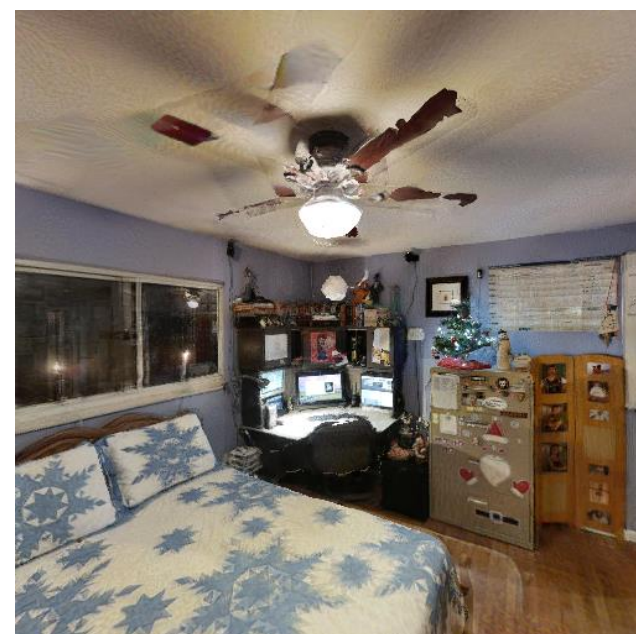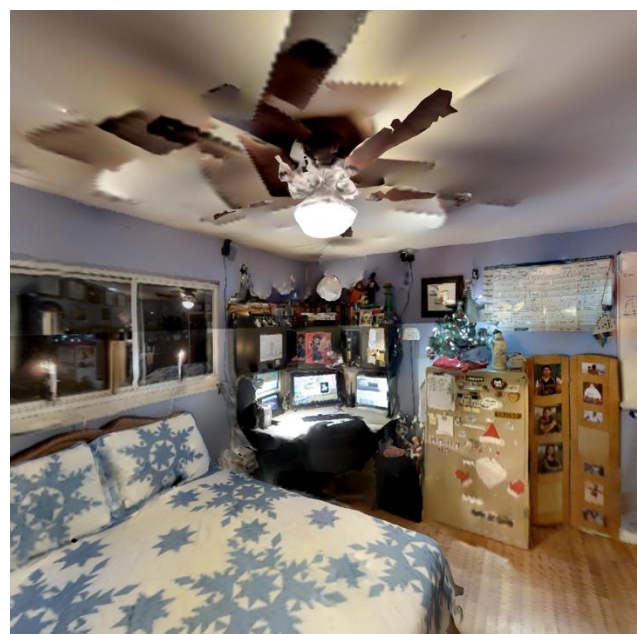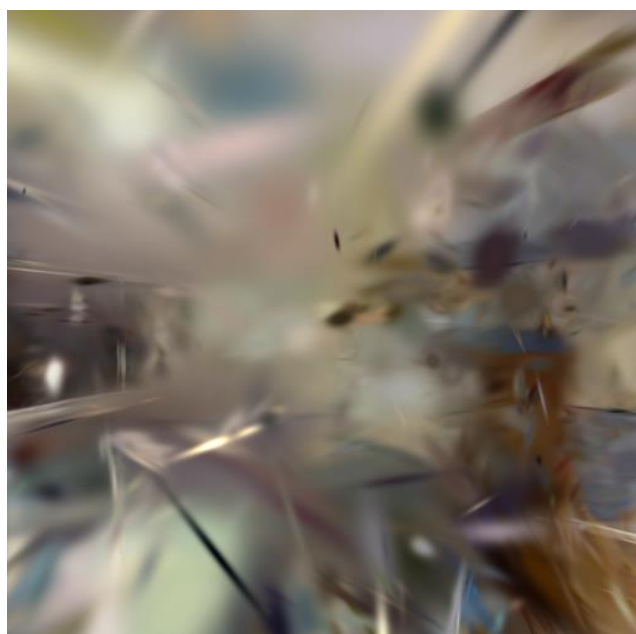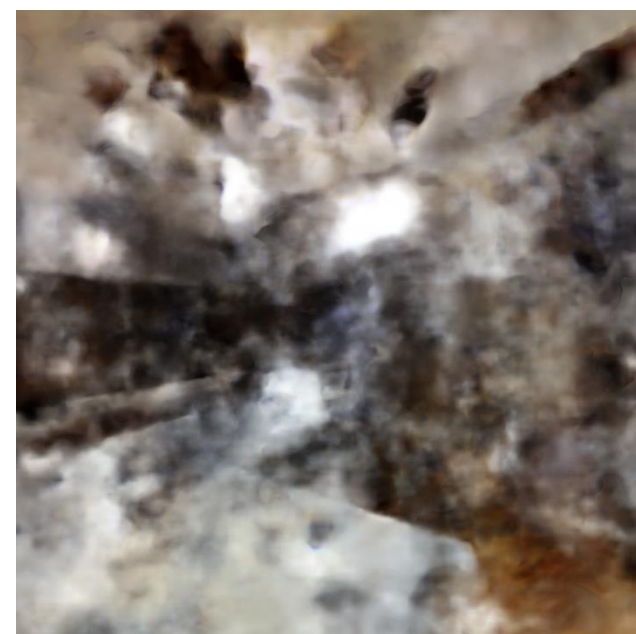

8194nk7LbLH

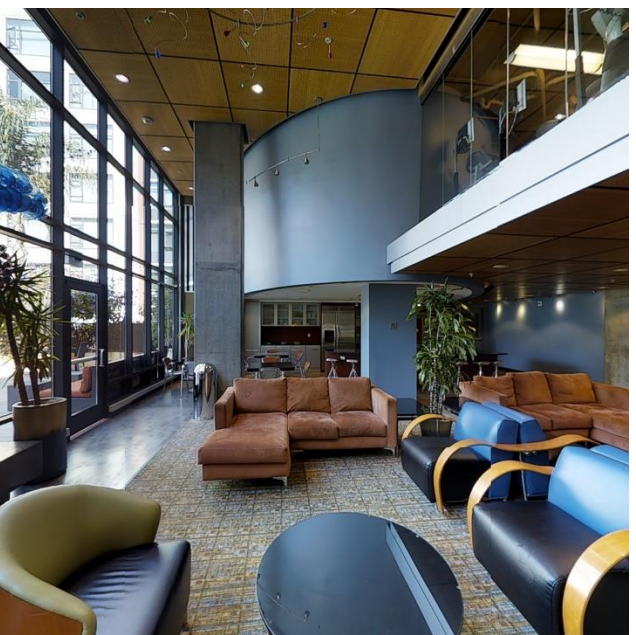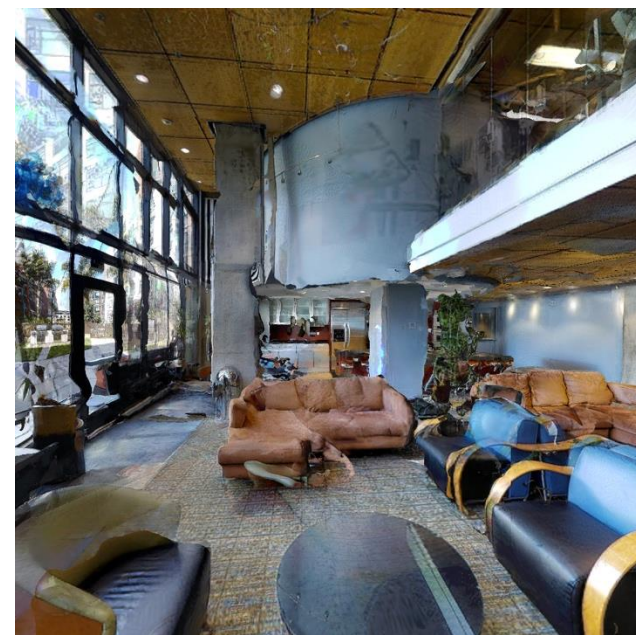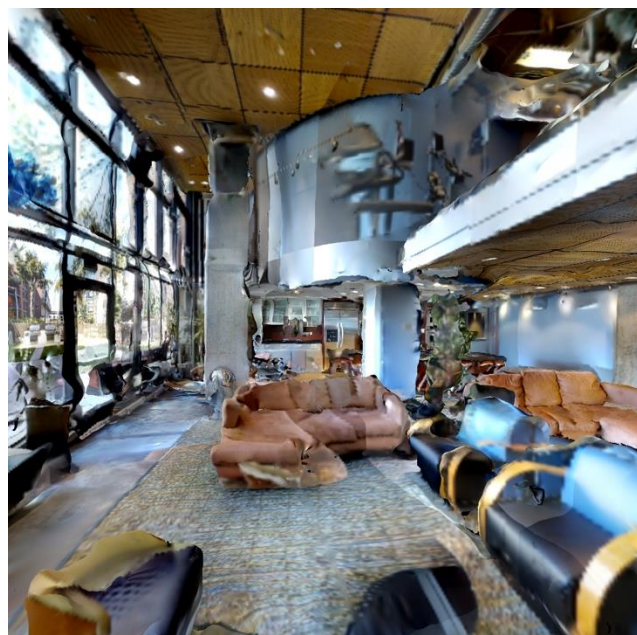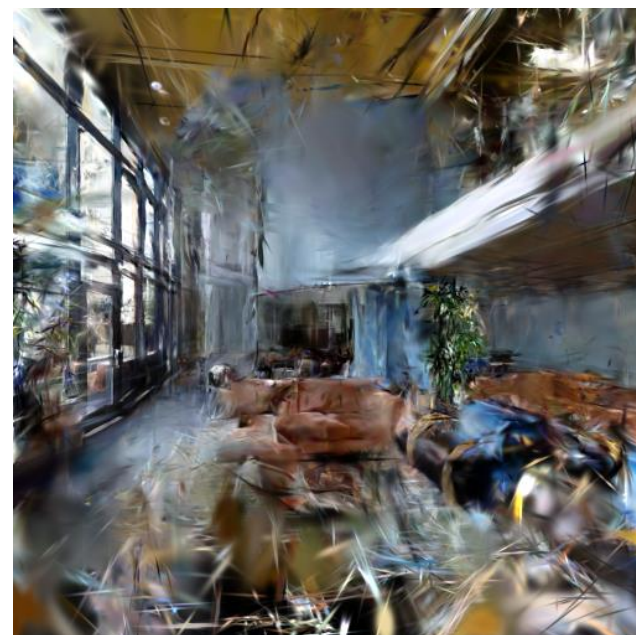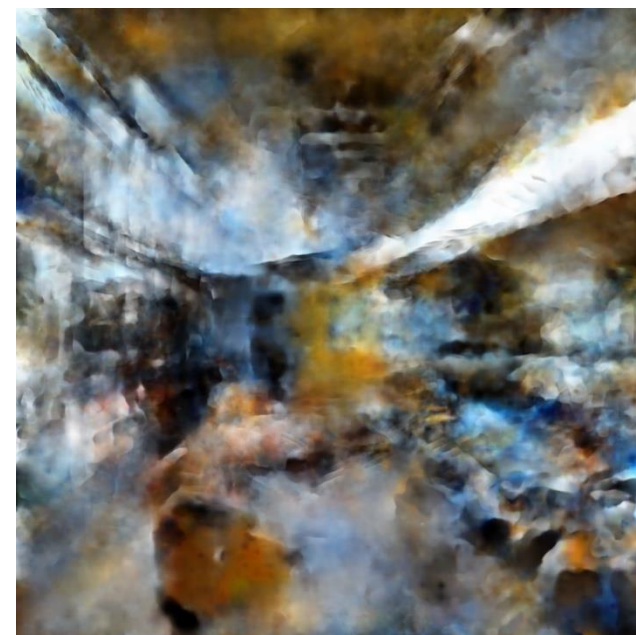

zsNo4HB9uLZ

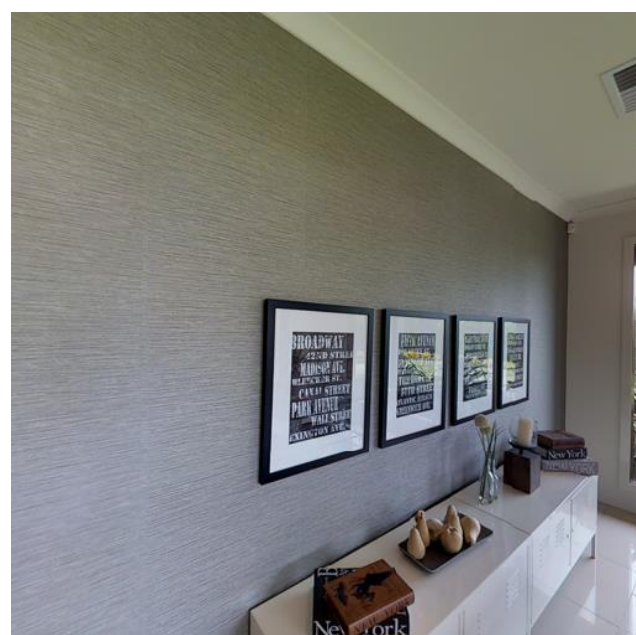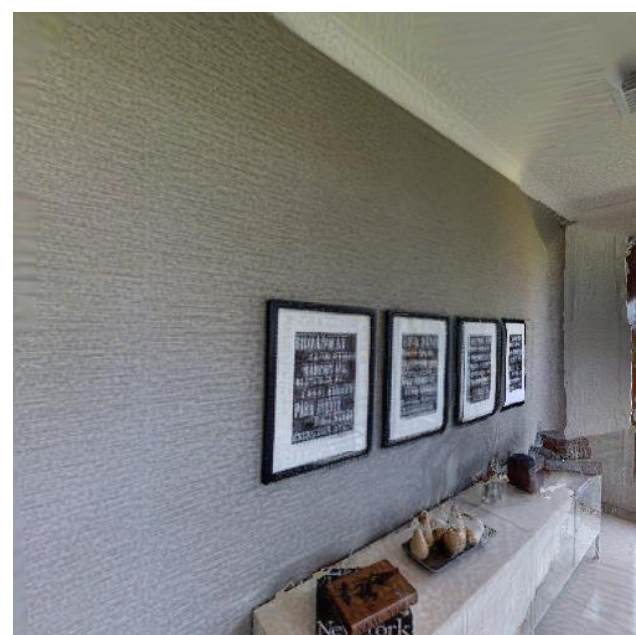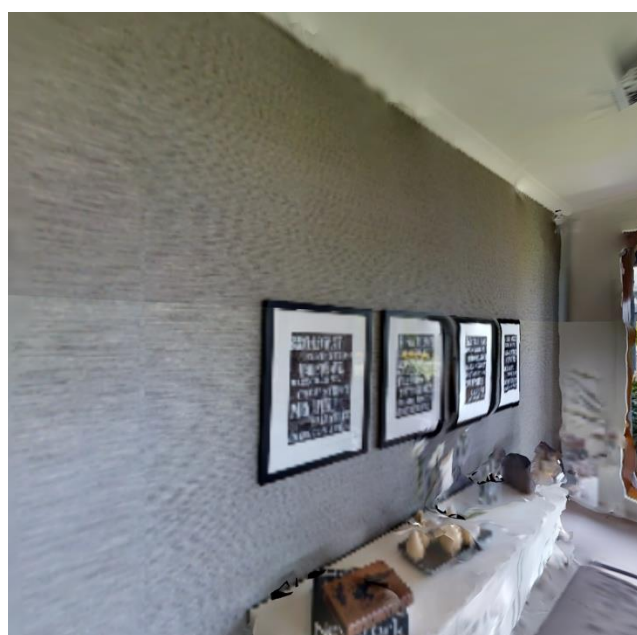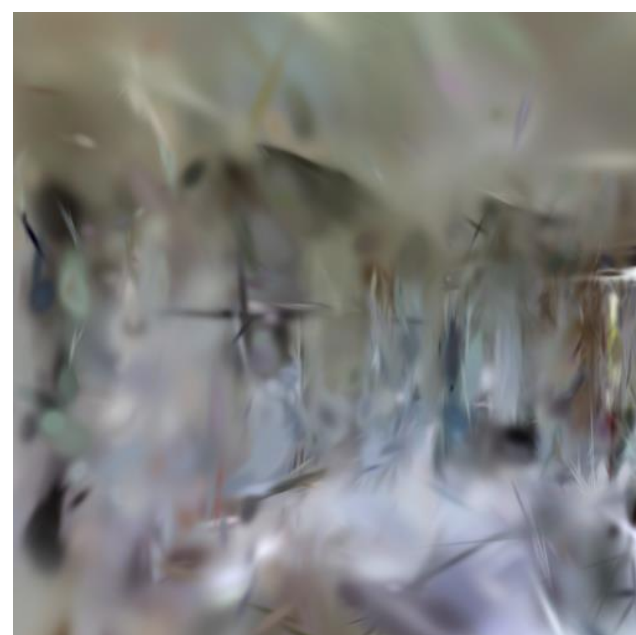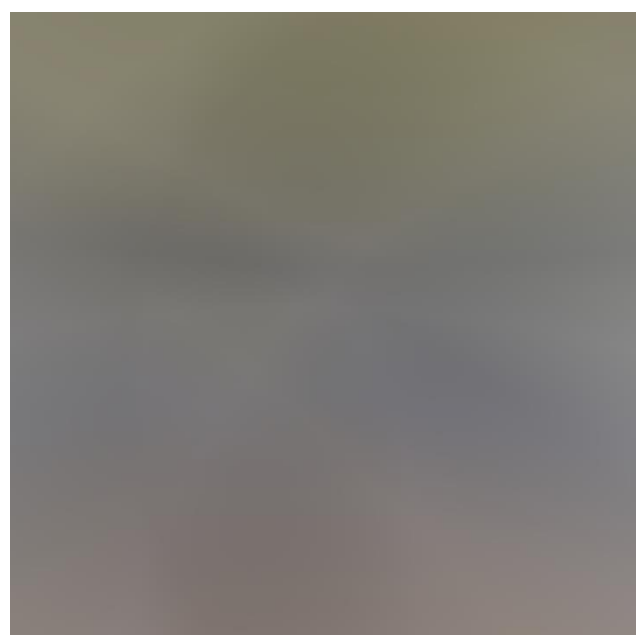

Scene

(a) Ours

(b) TexRecon

(c) SparseGS

(d) ZipNeRF

2t7WUuJeko7

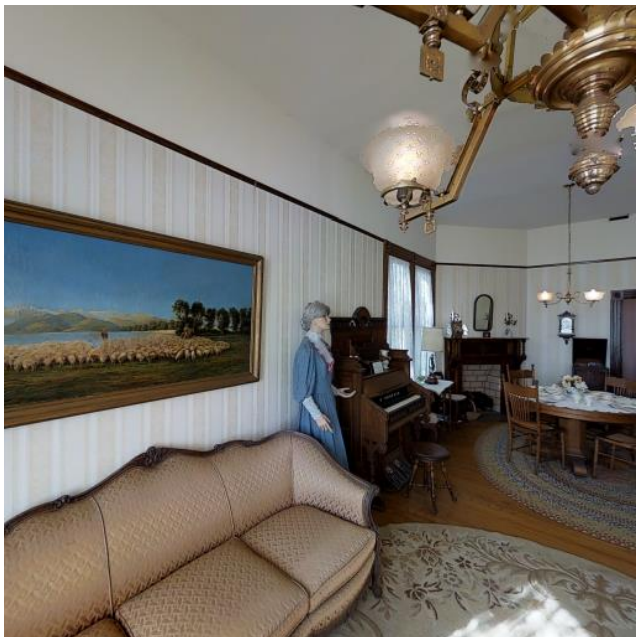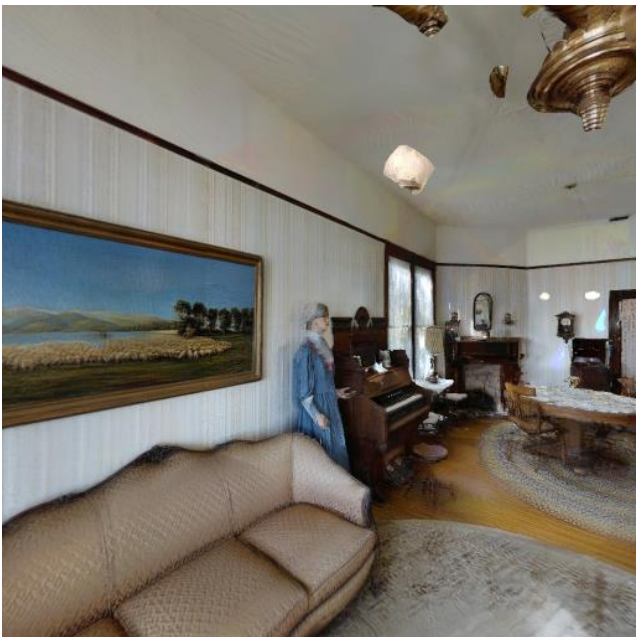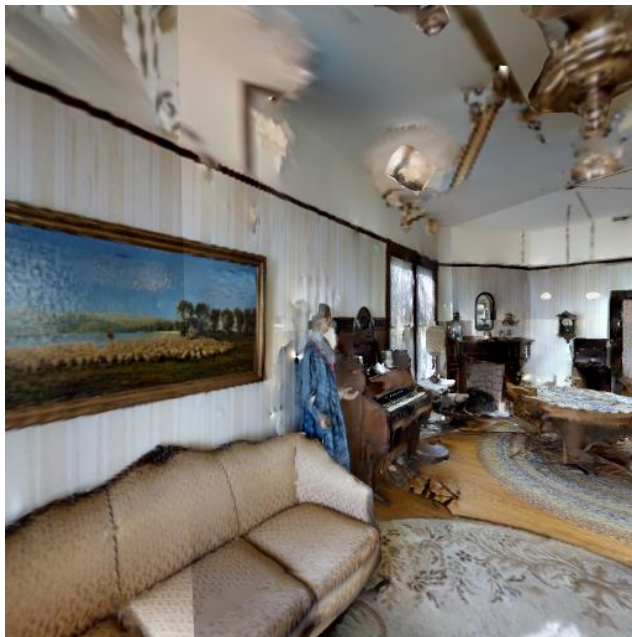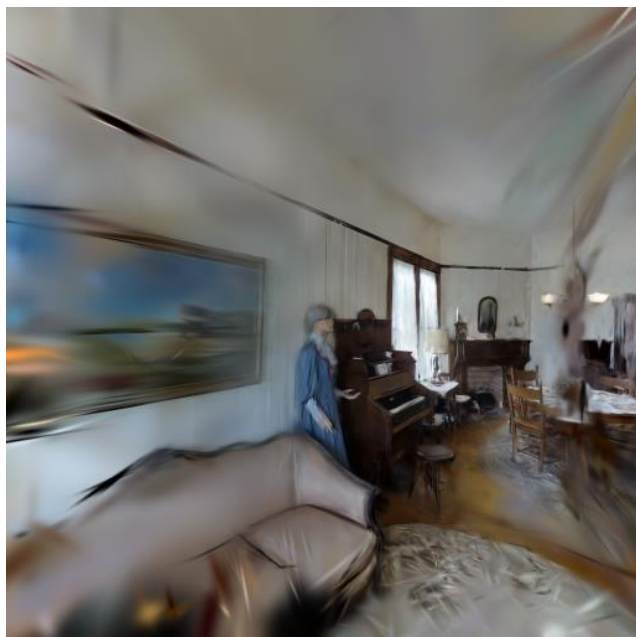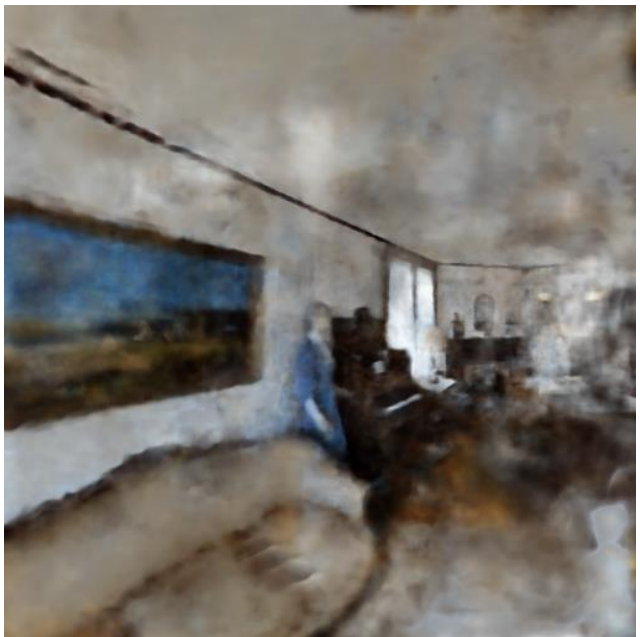

YVUC4YcDtcY

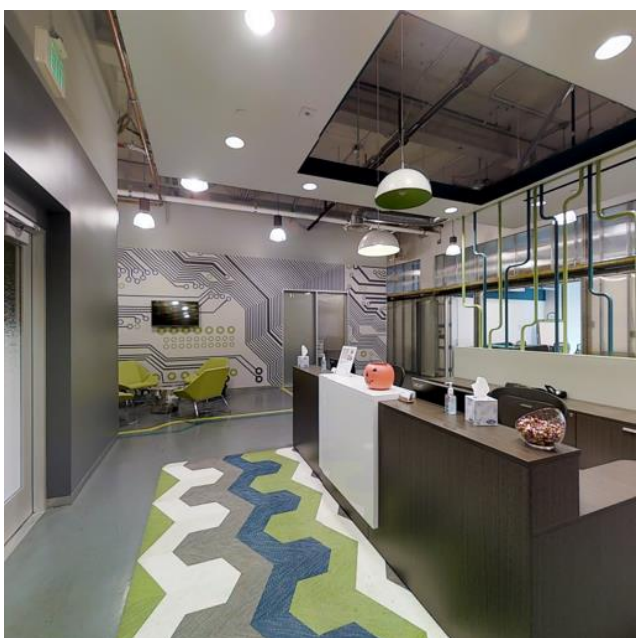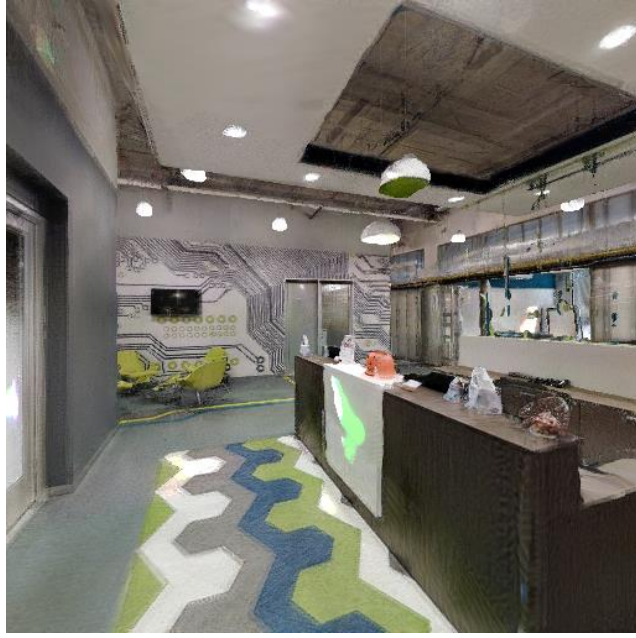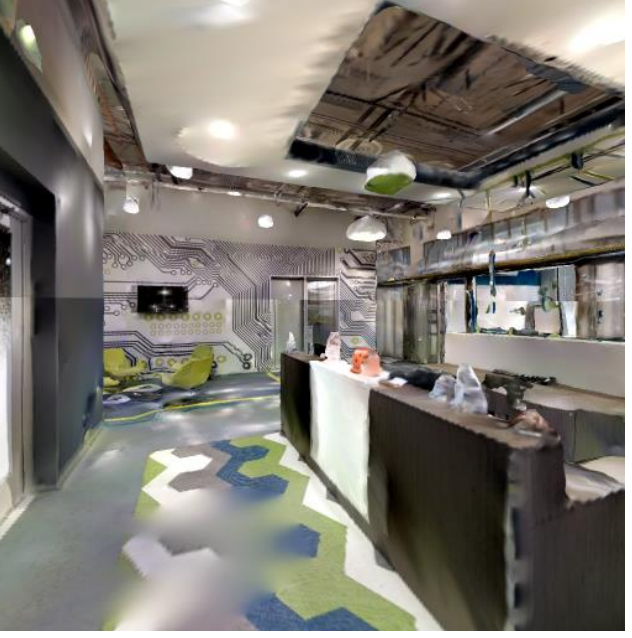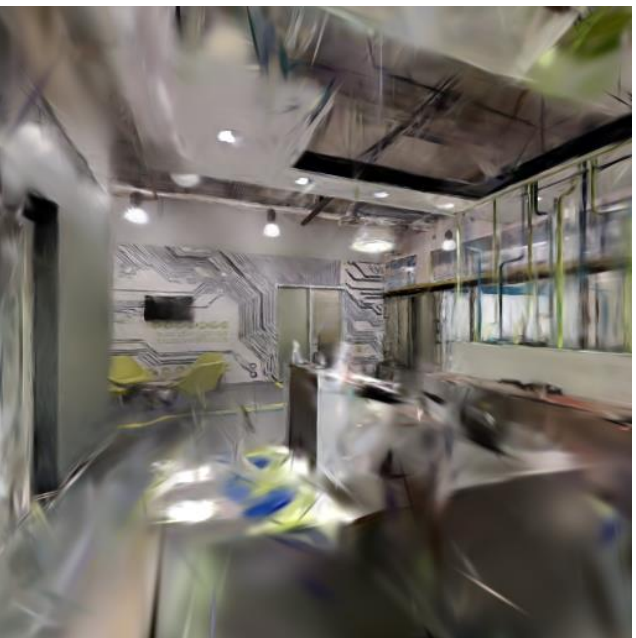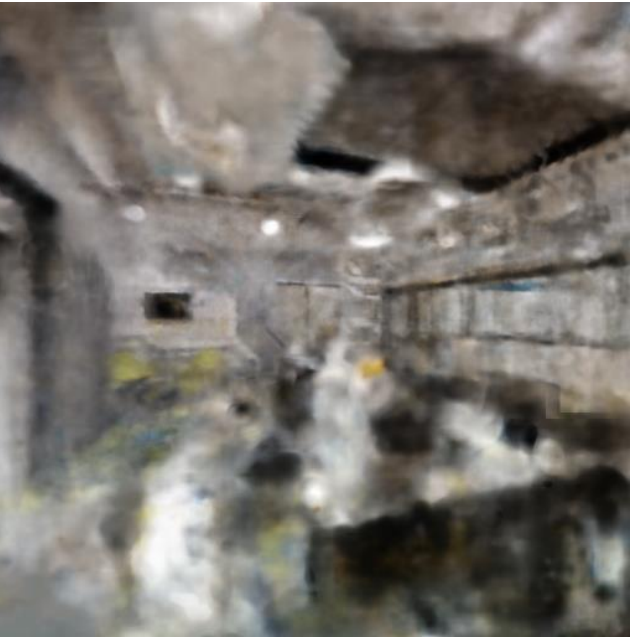

pLe4wQe7qrG

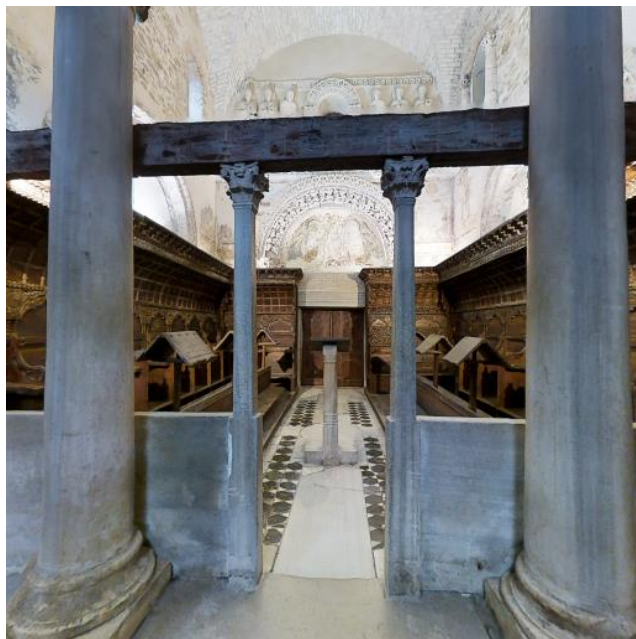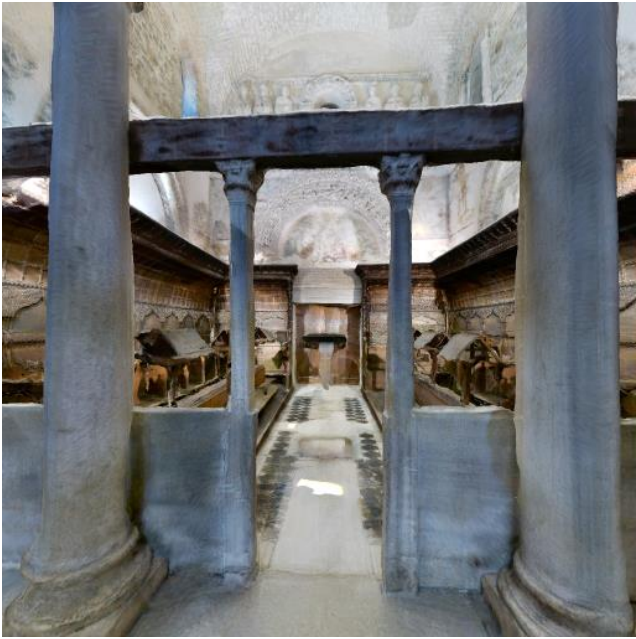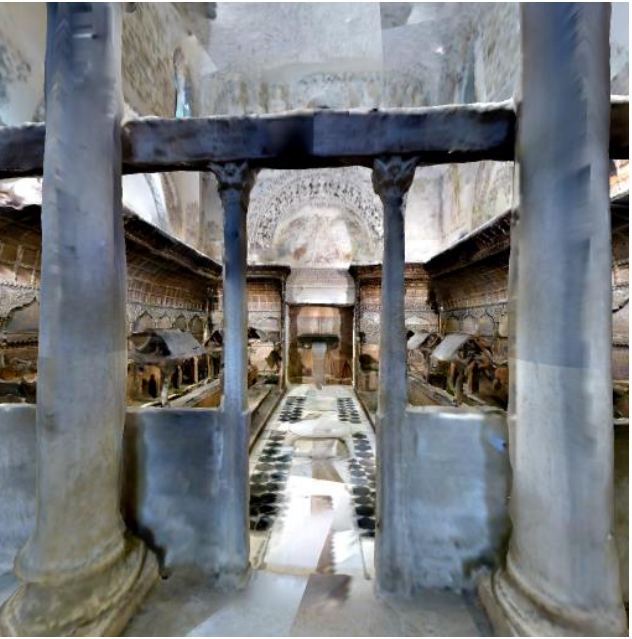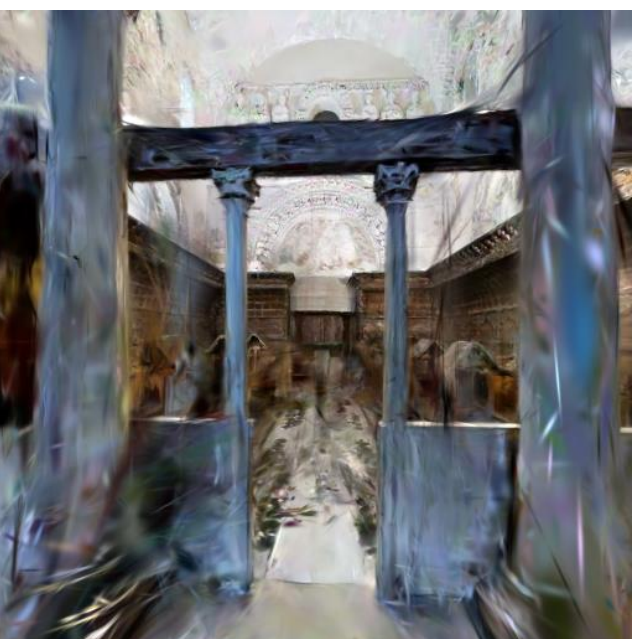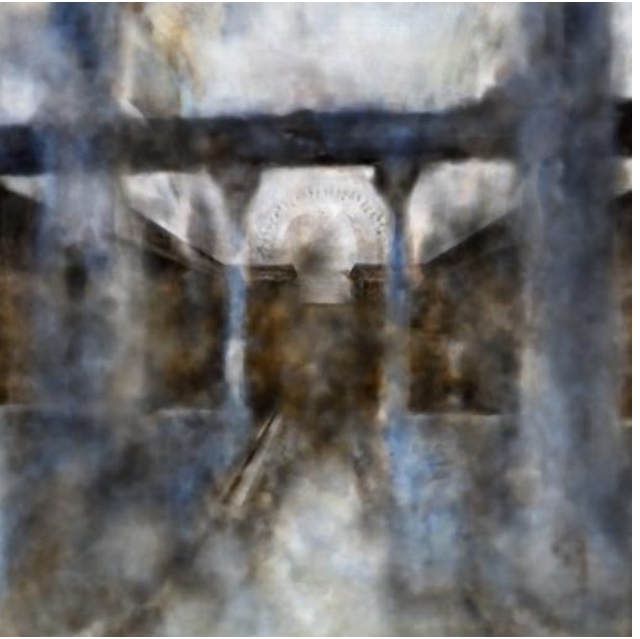

RPmz2sHmrrY

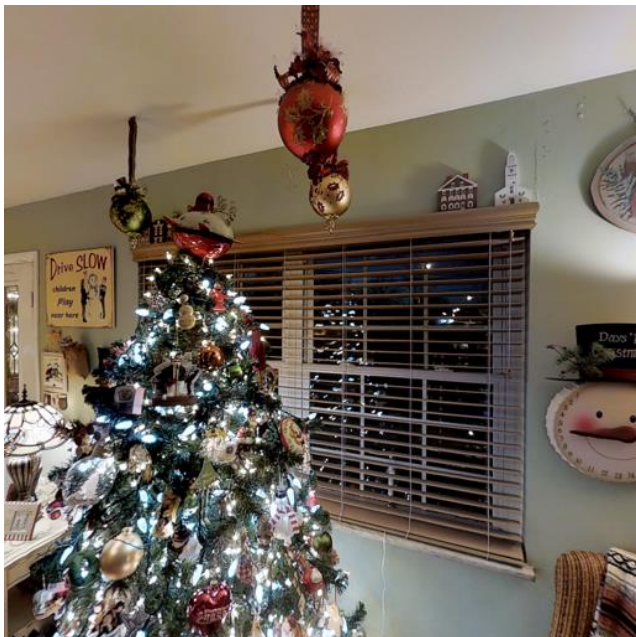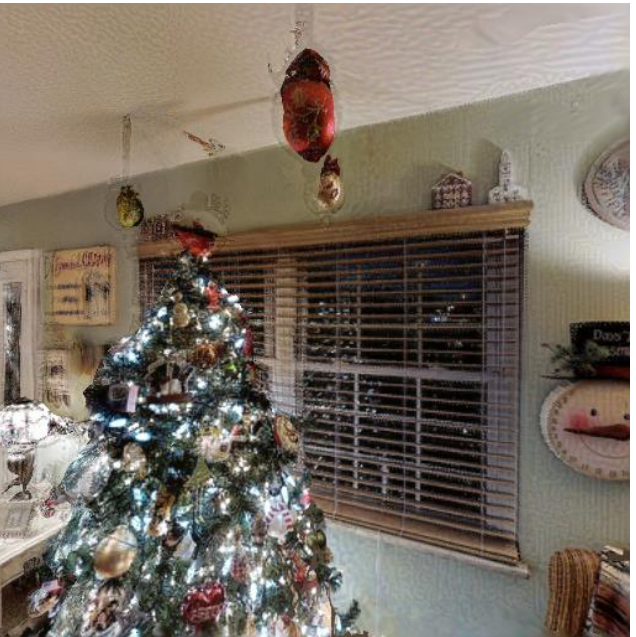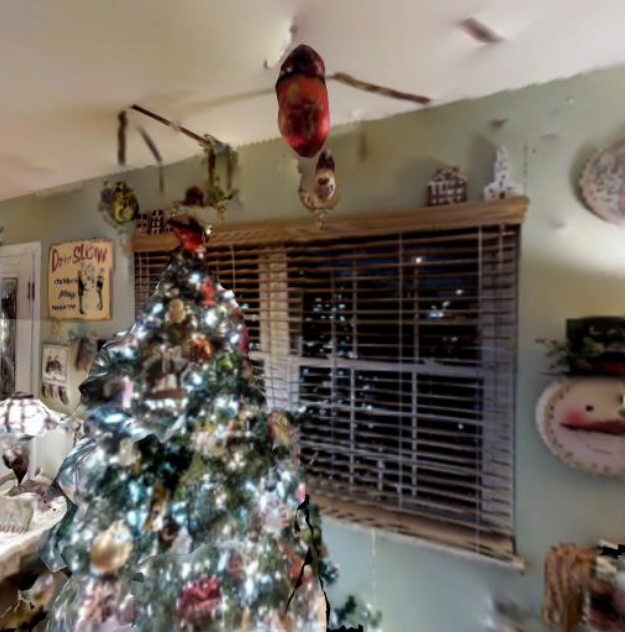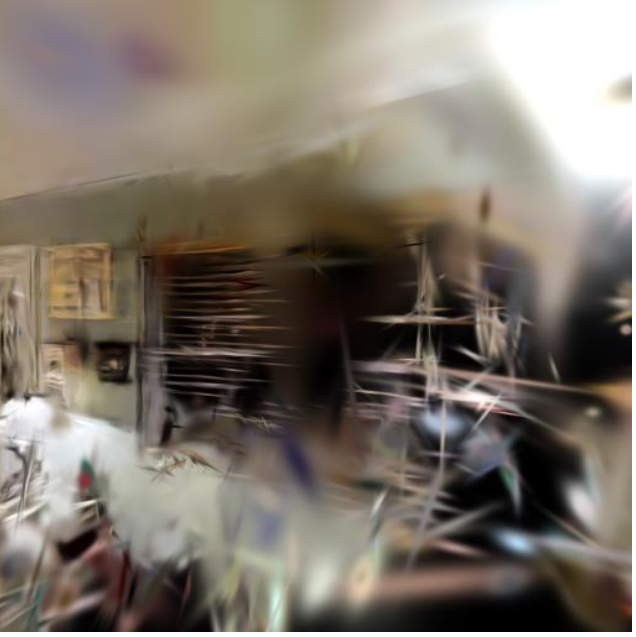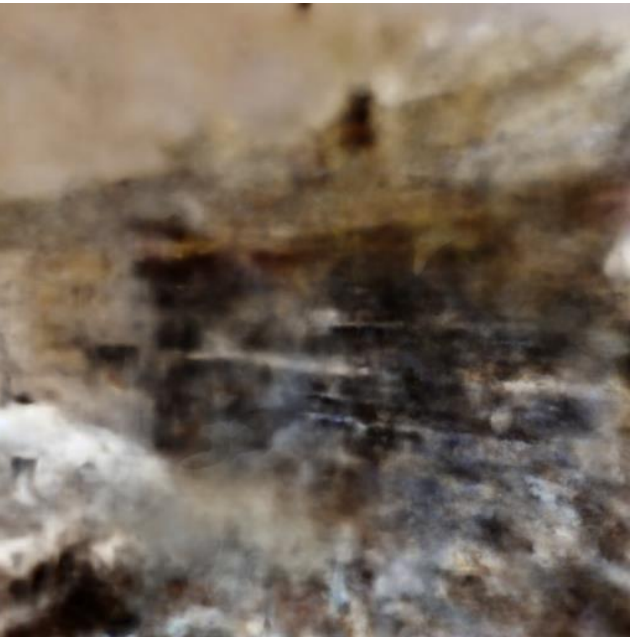

8194nk7LbLH

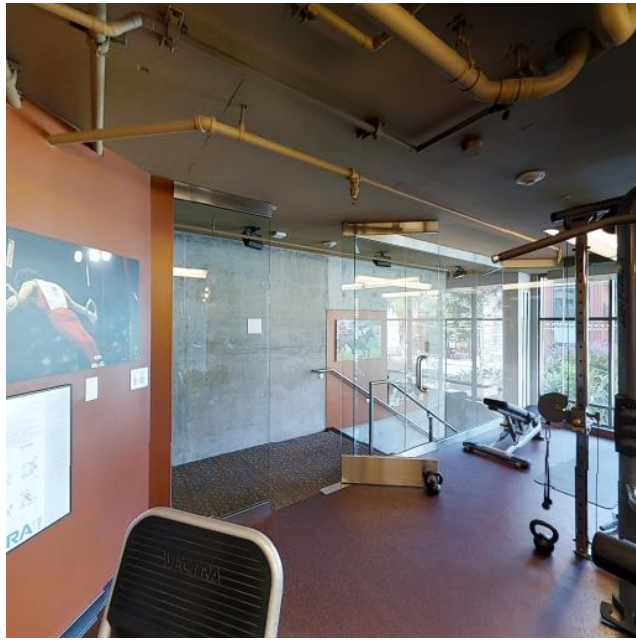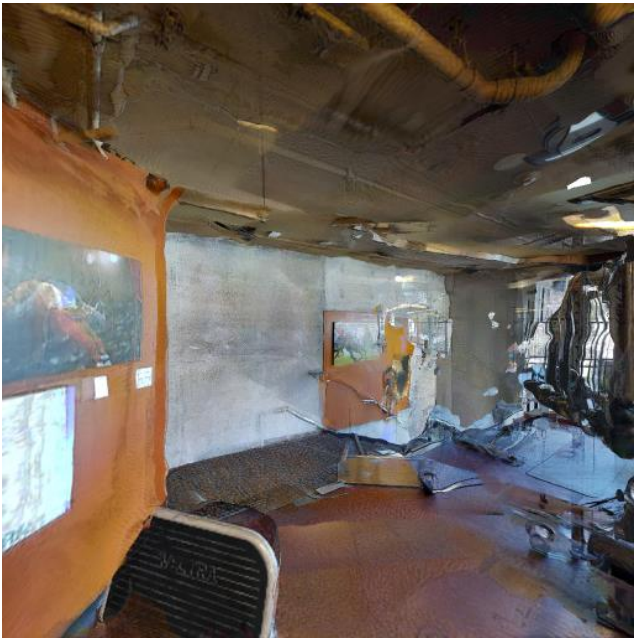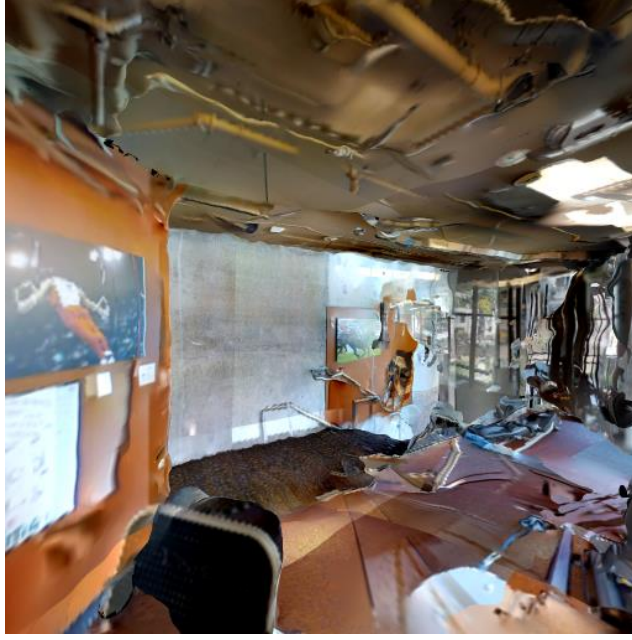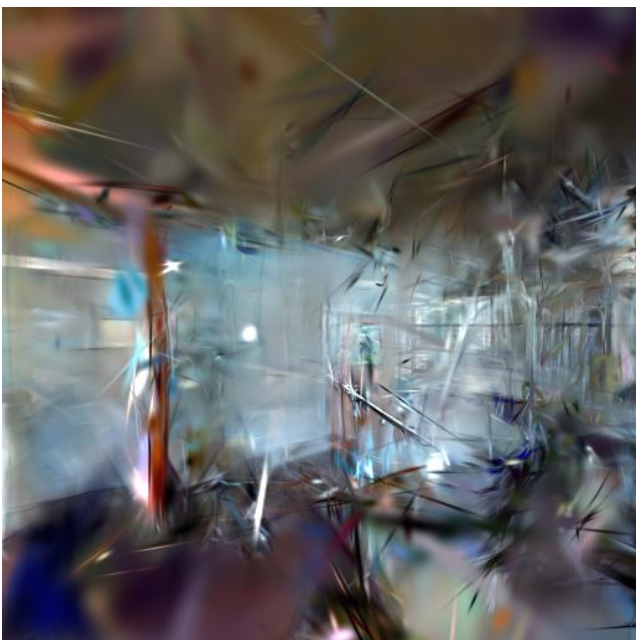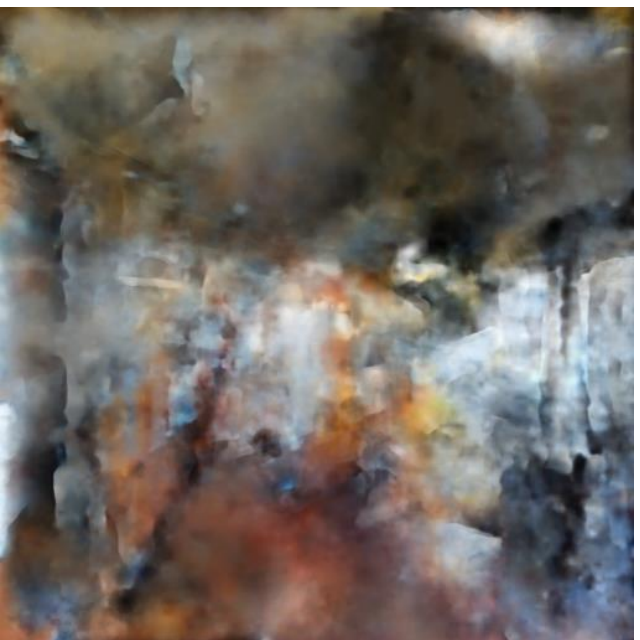

zsNo4HB9uLZ

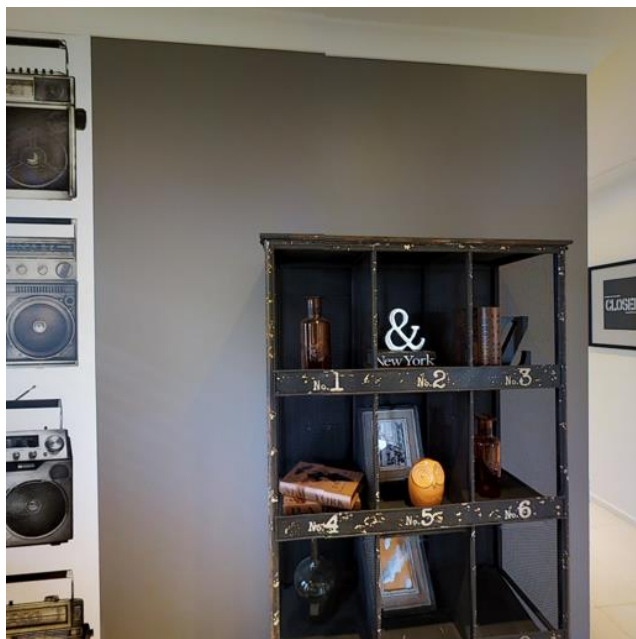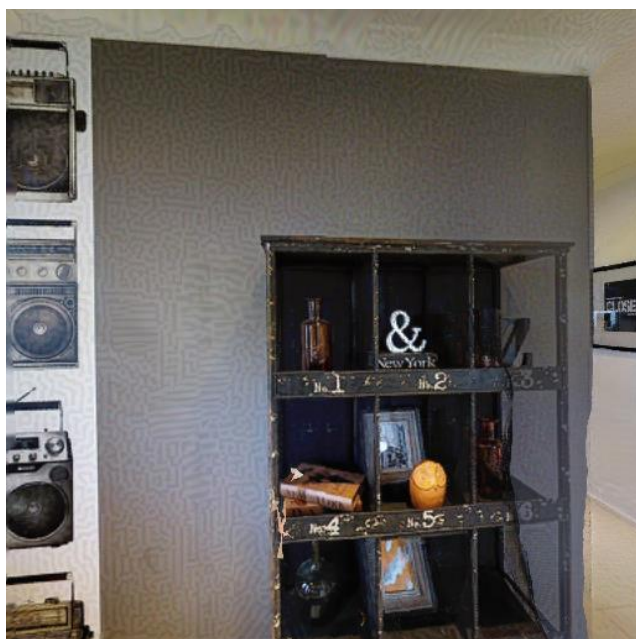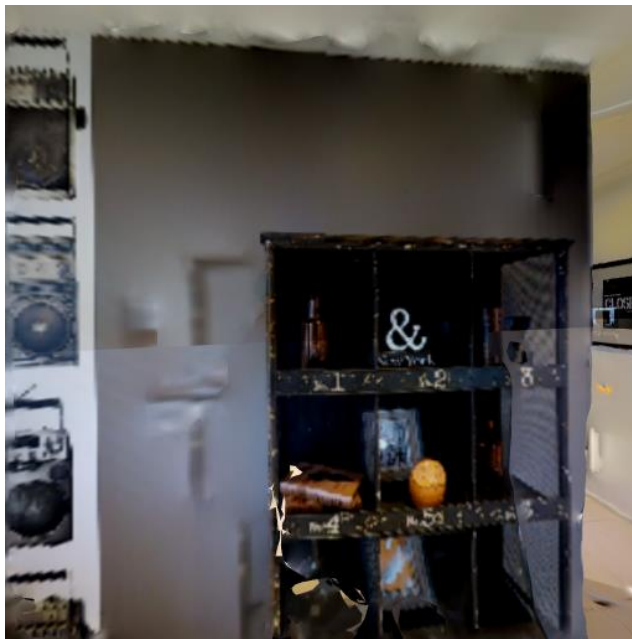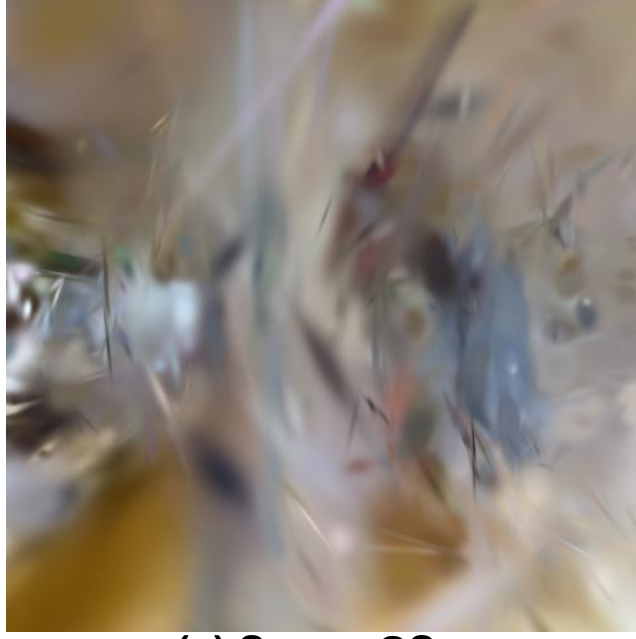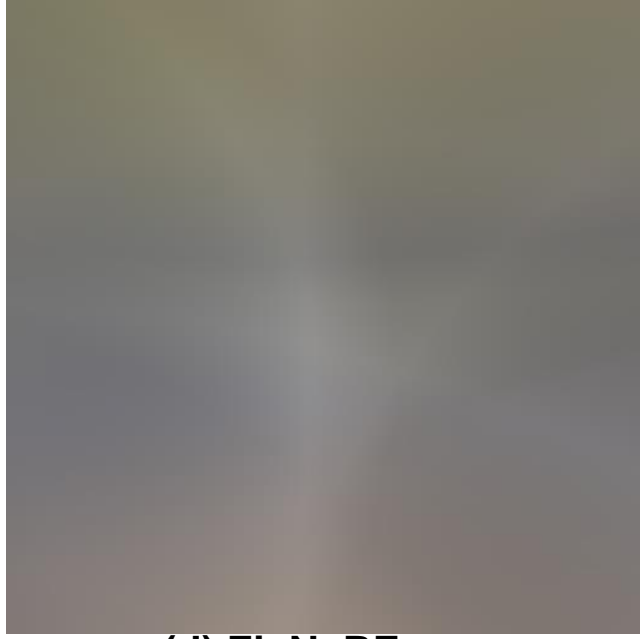

Scene

(a) Ours

(b) TexRecon

(c) SparseGS

(d) ZipNeRF

2t7WUuJeko7

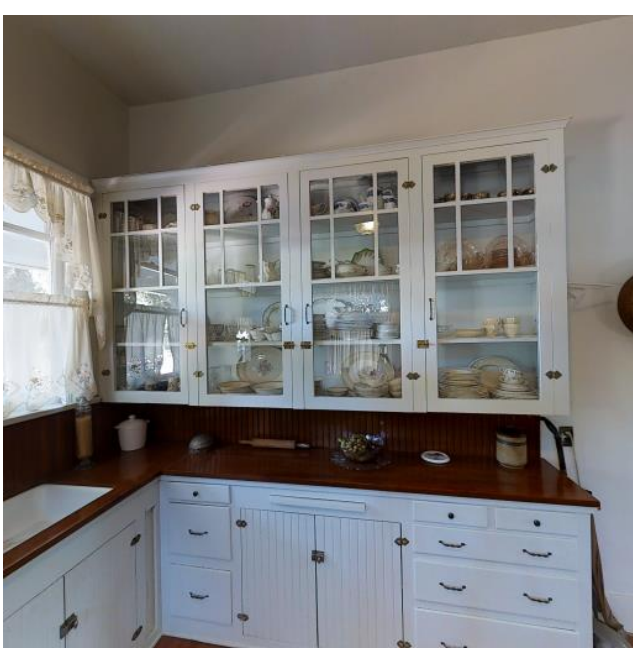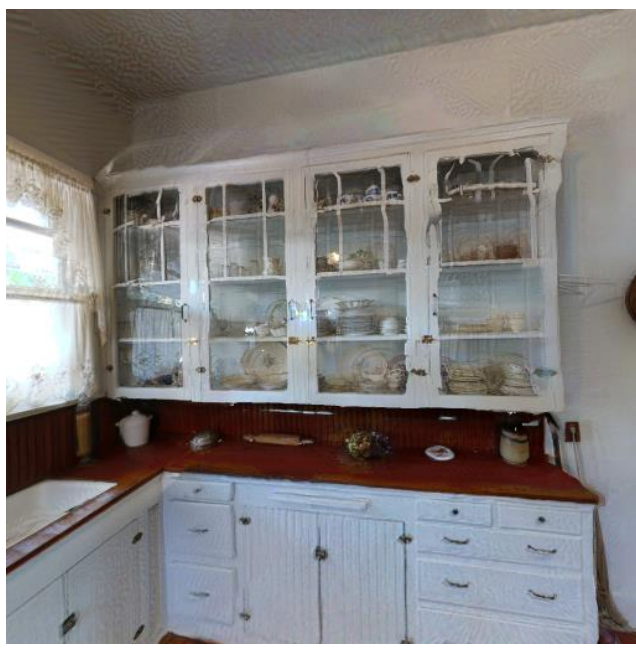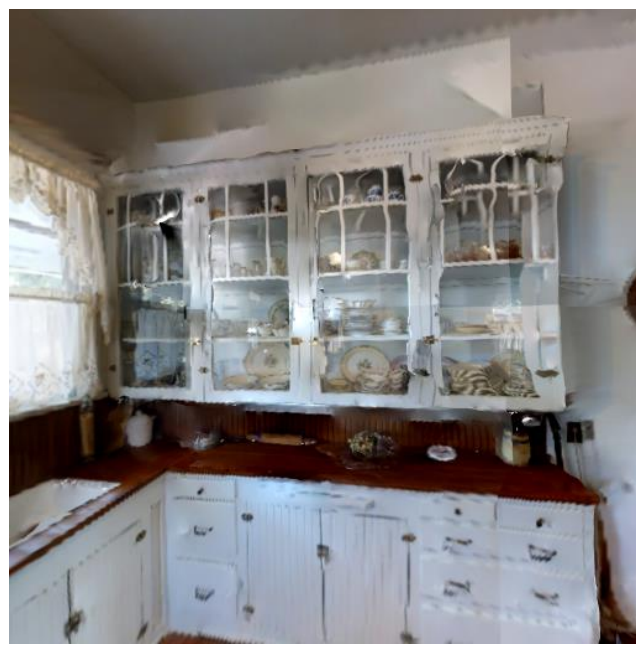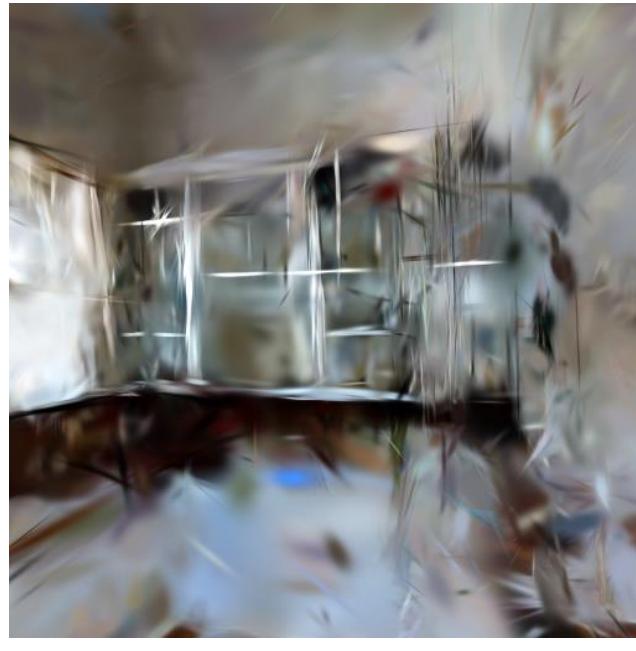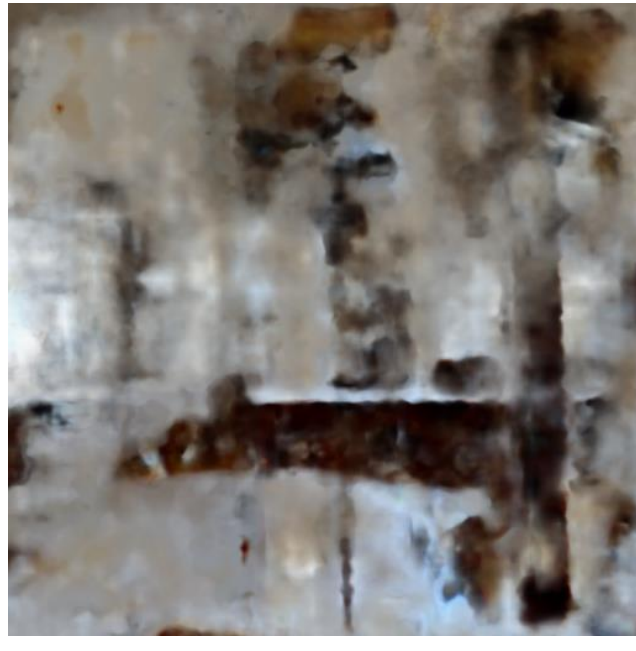

YVUC4YcDtcY

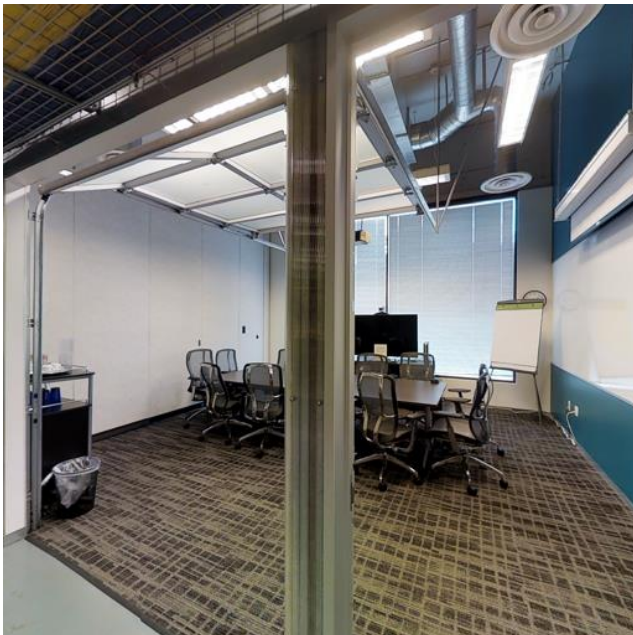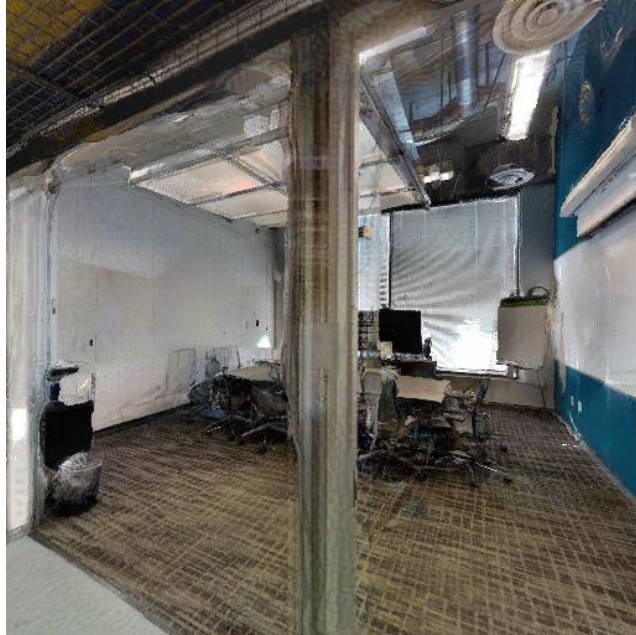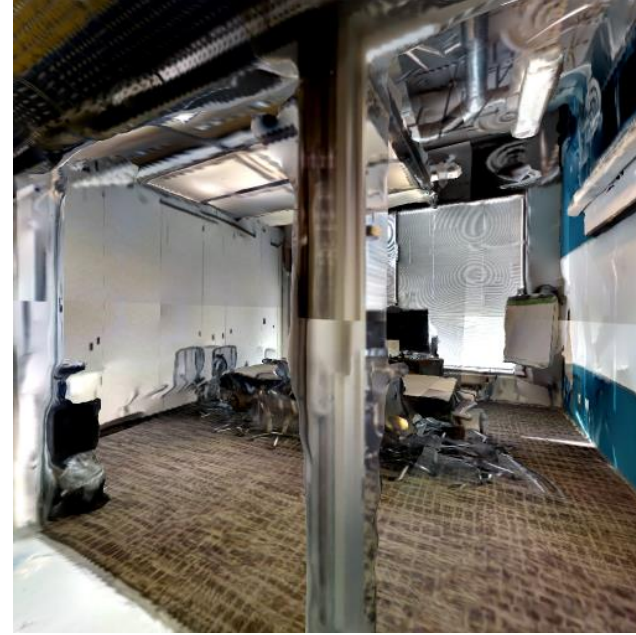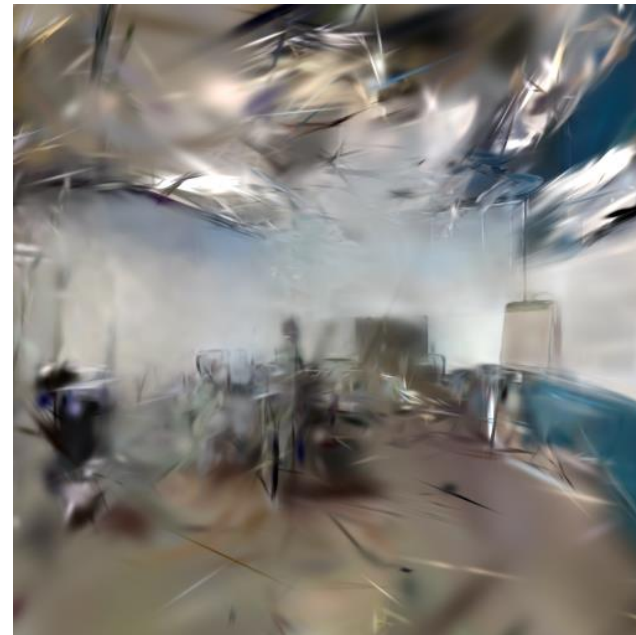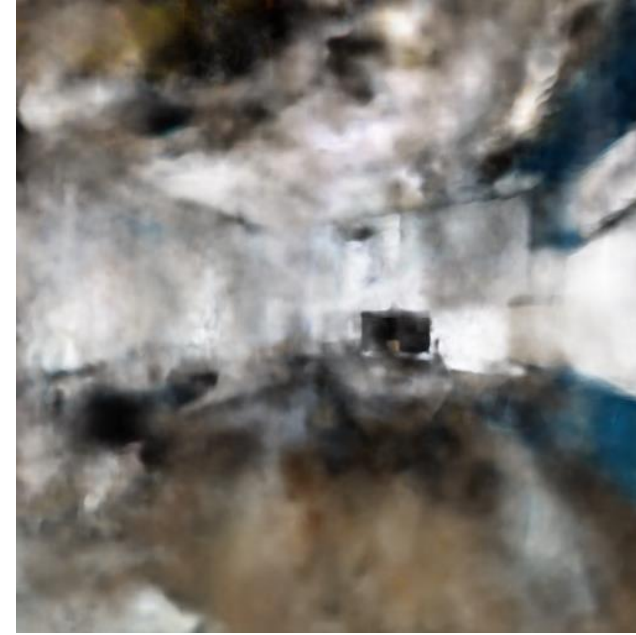

pLe4wQe7qrG

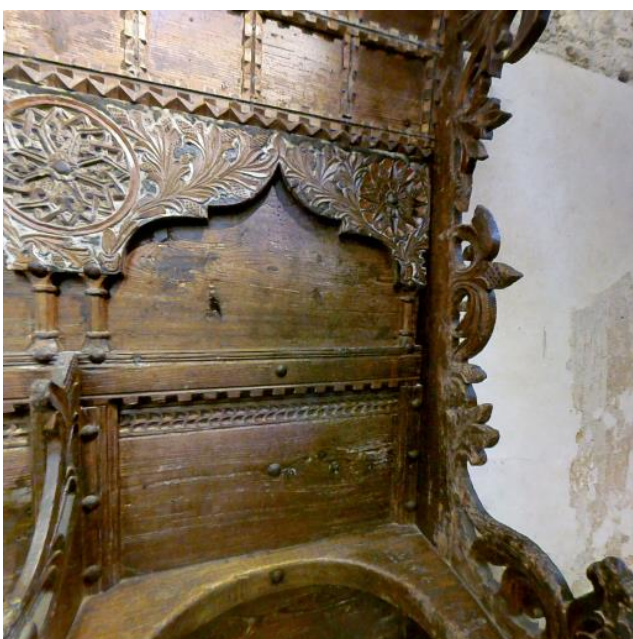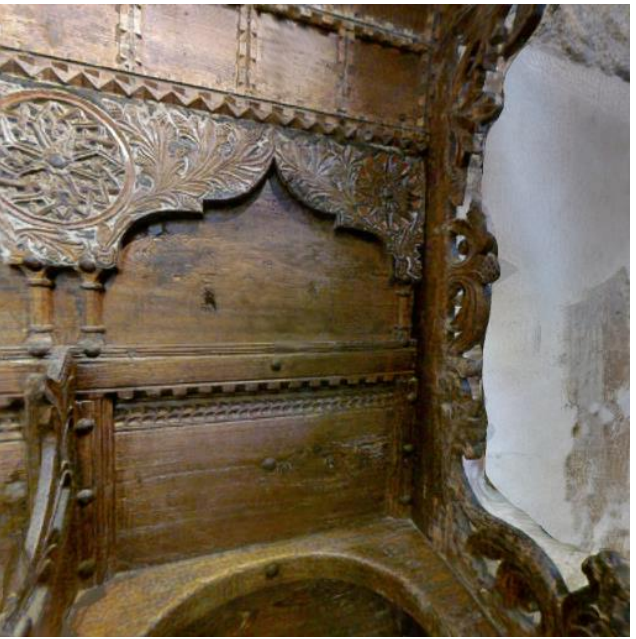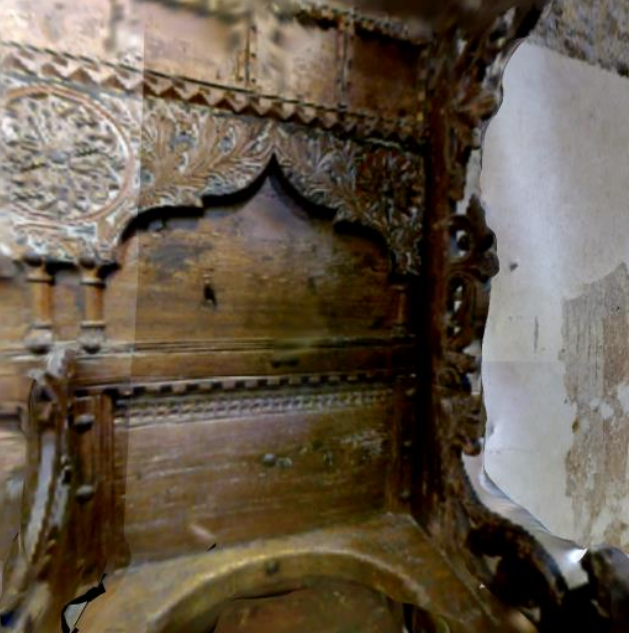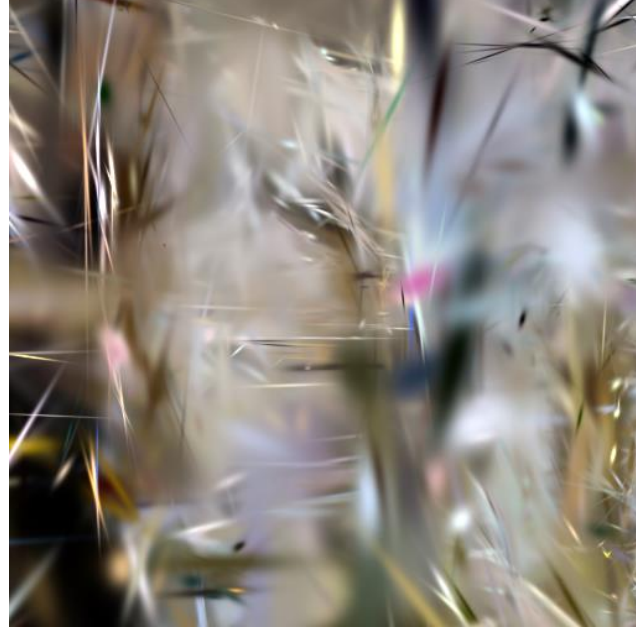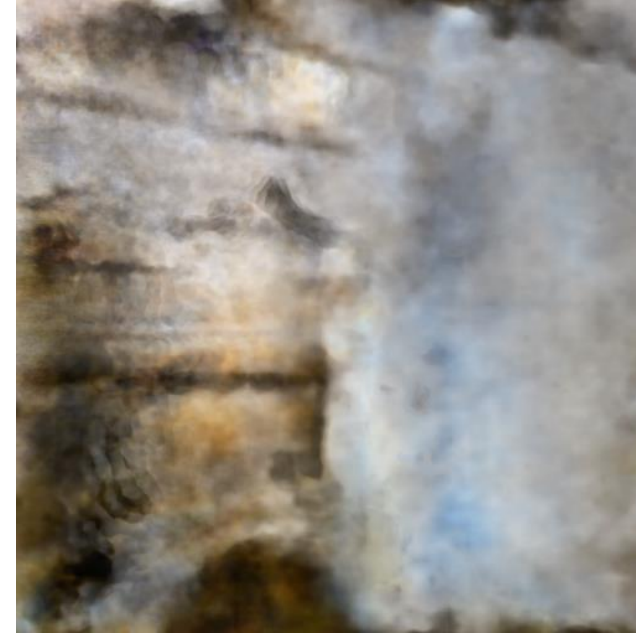

RPmz2sHmrrY

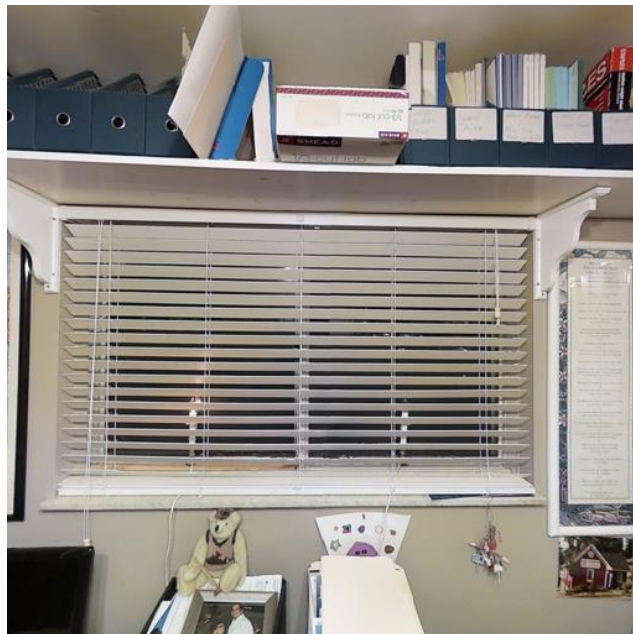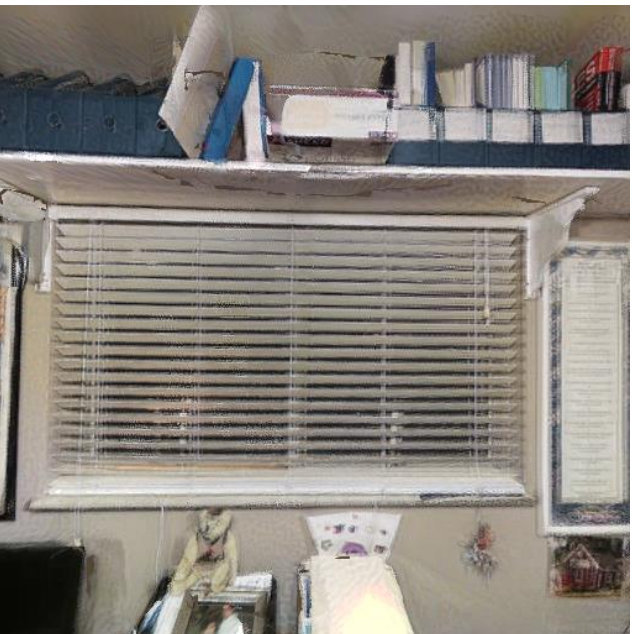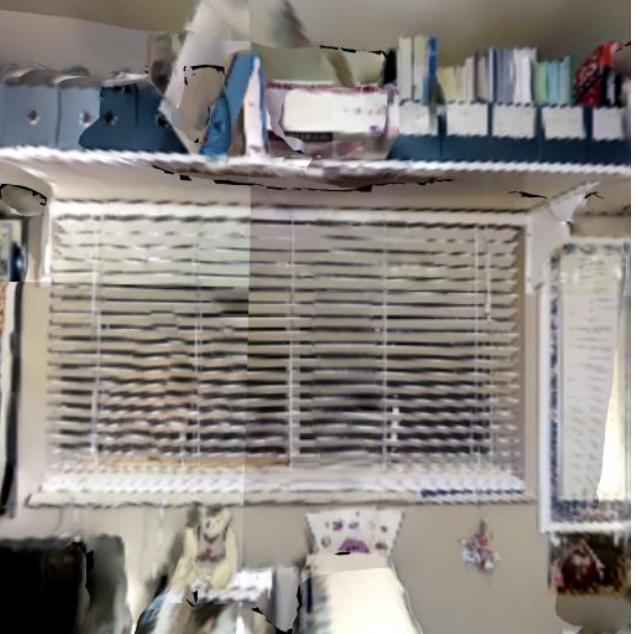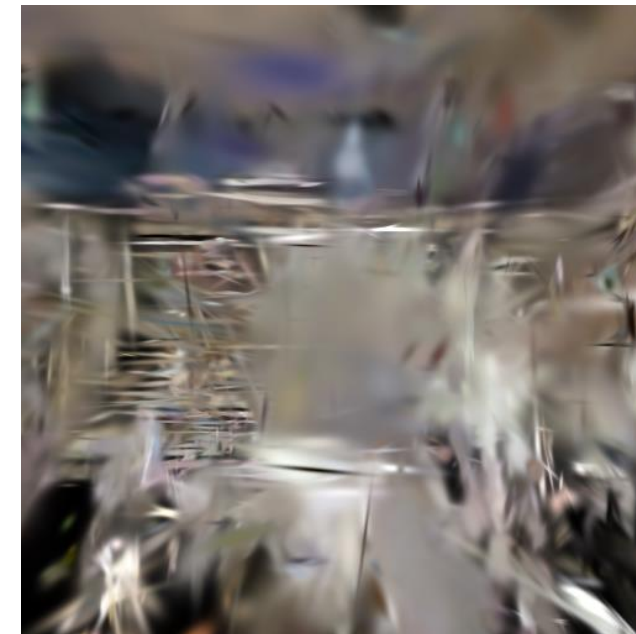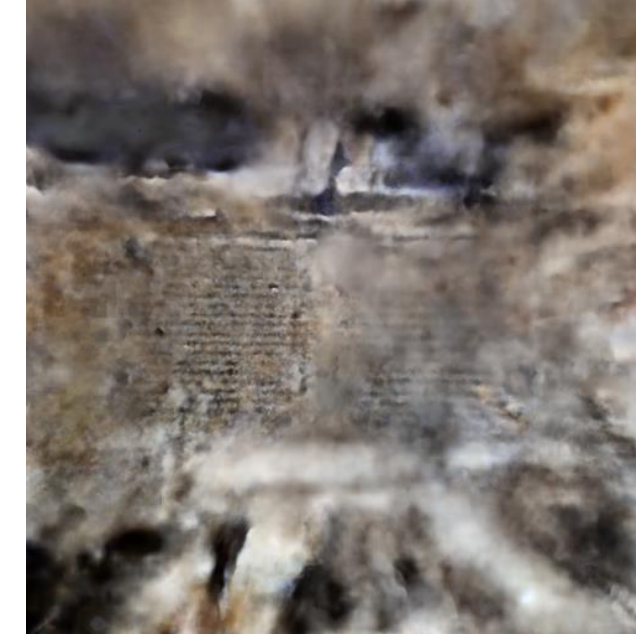

8194nk7LbLH

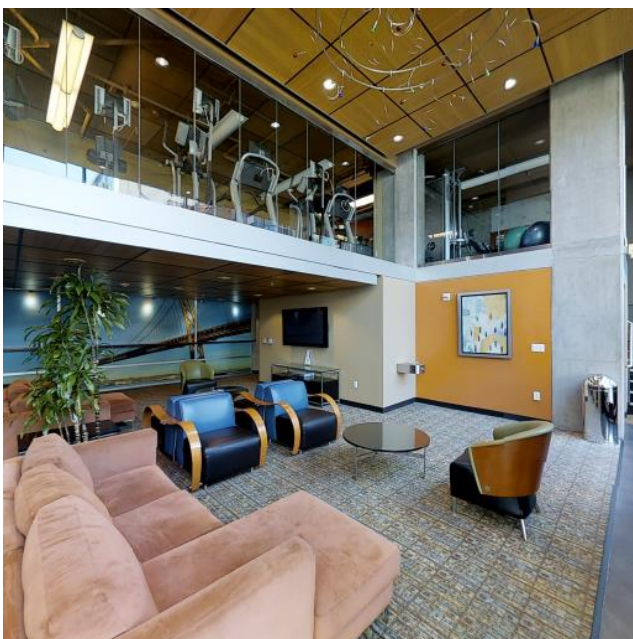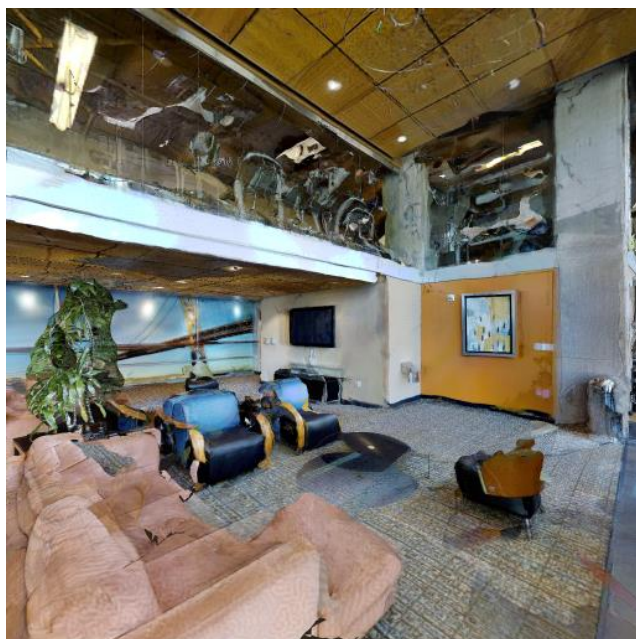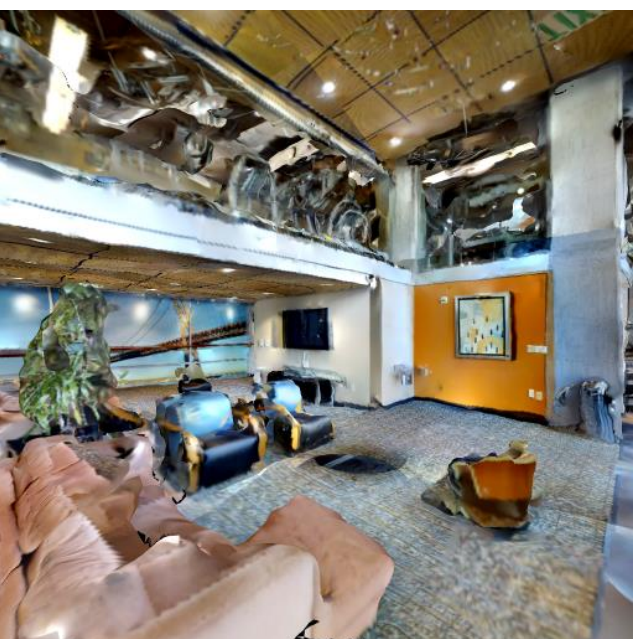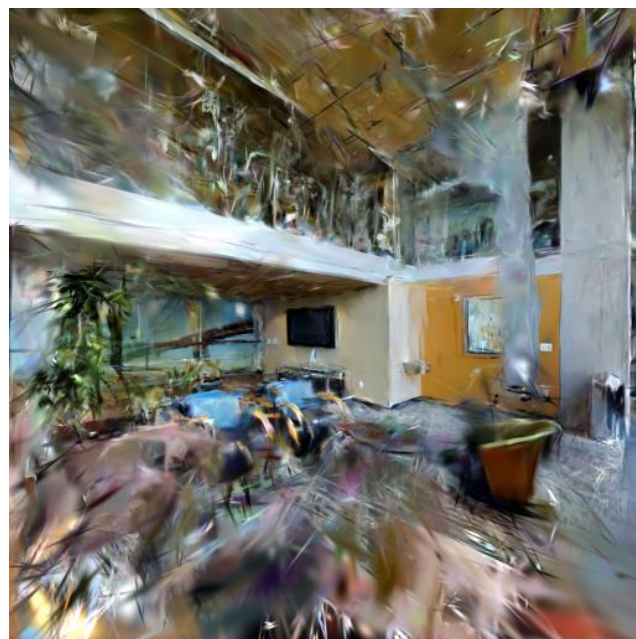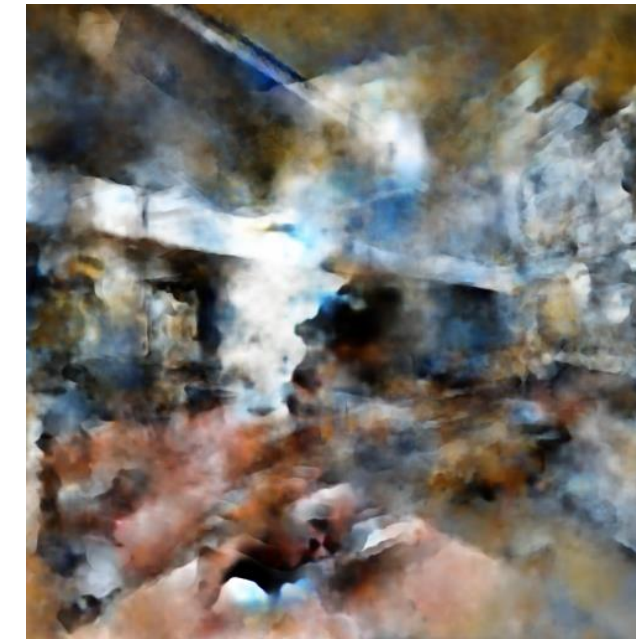

zsNo4HB9uLZ

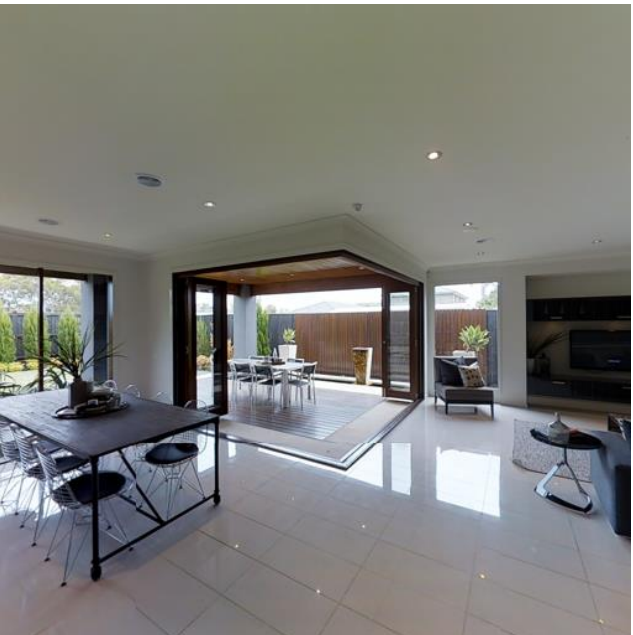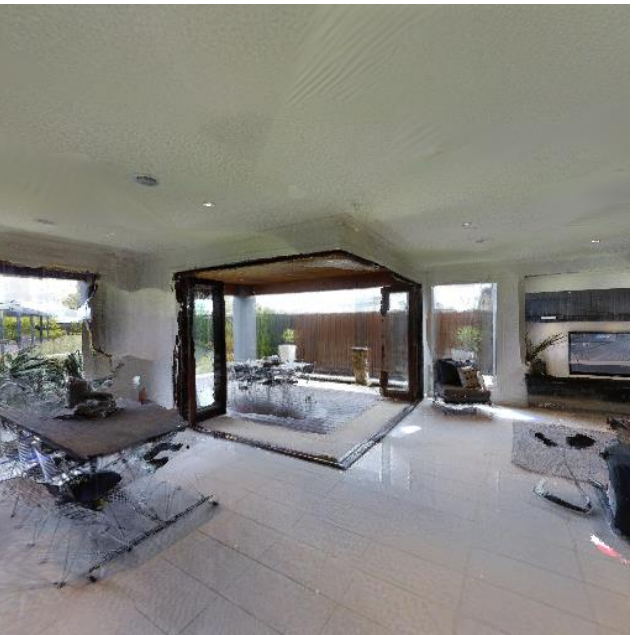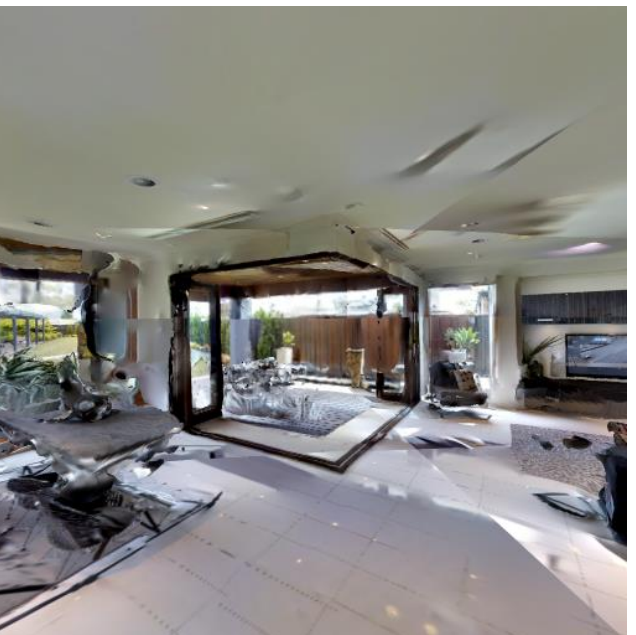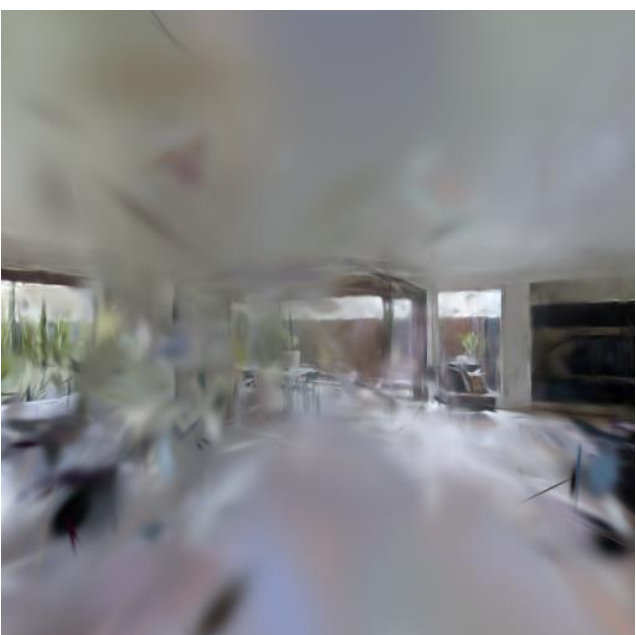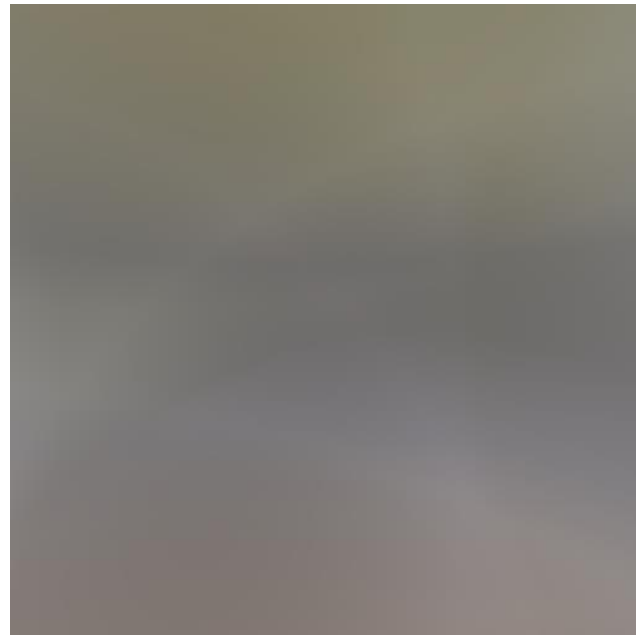

Scene

(a) Ours

(b) TexRecon

(c) SparseGS

(d) ZipNeRF

2t7WUuJeko7

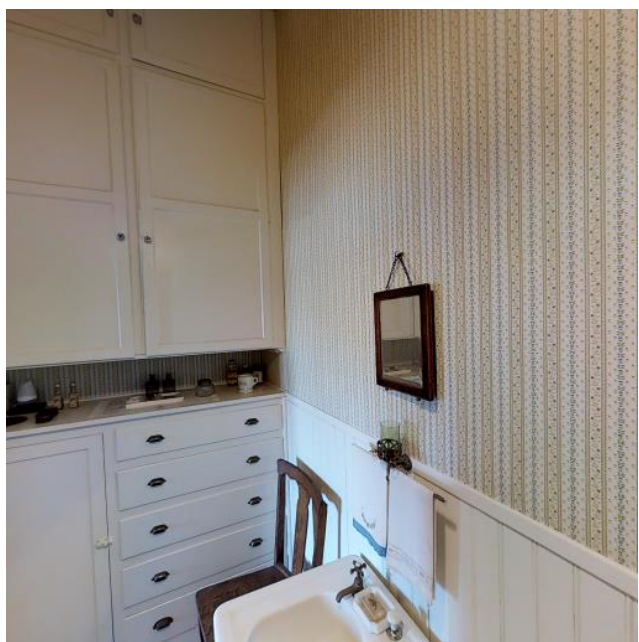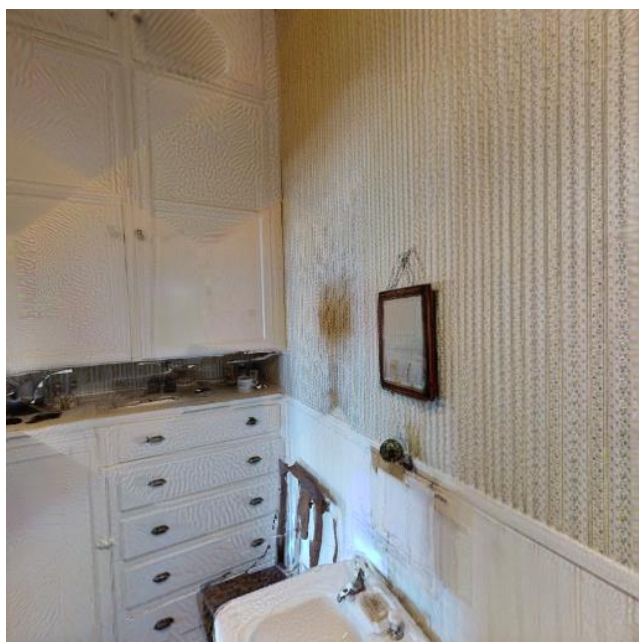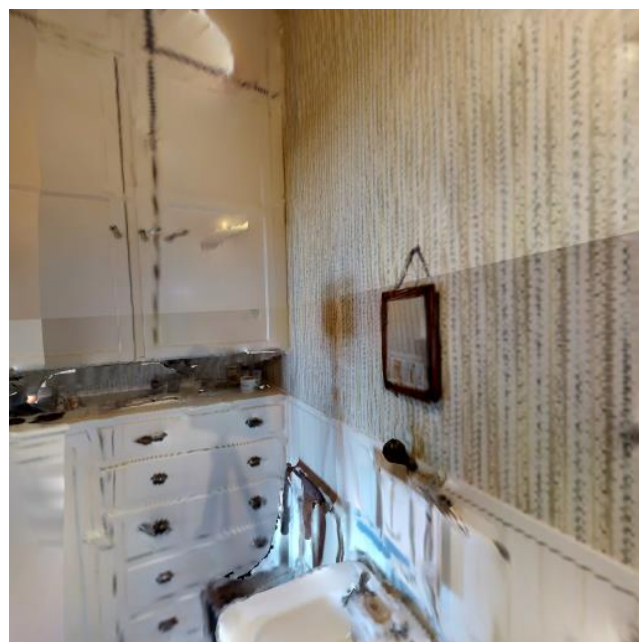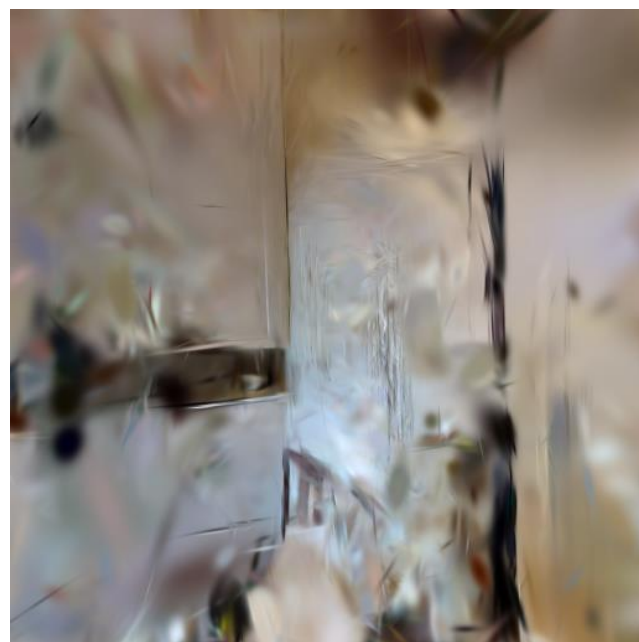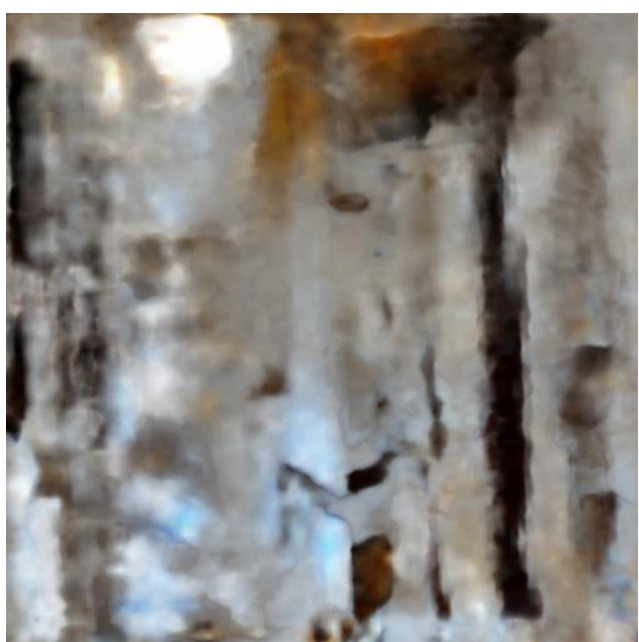

YVUC4YcDtcY

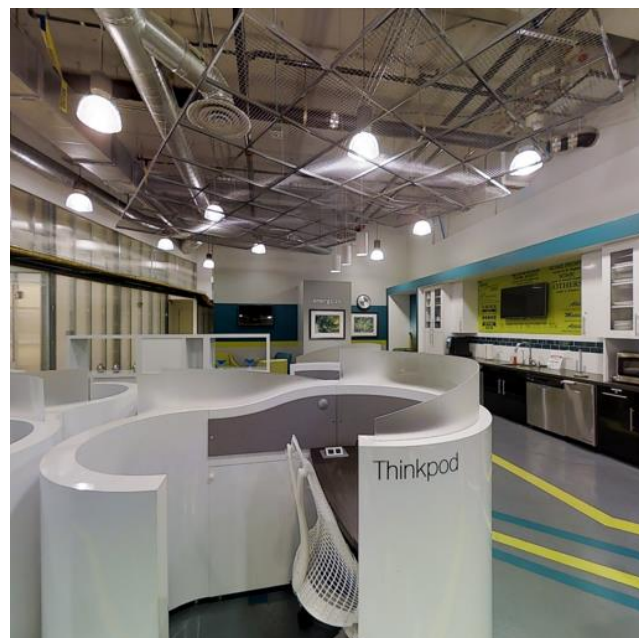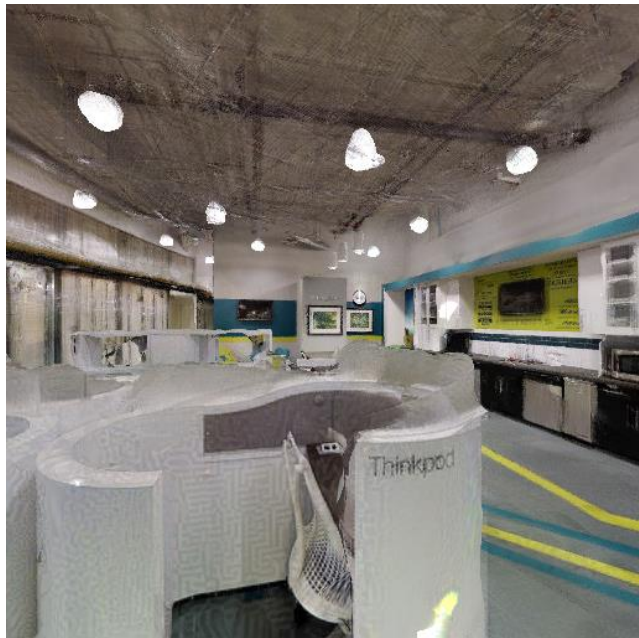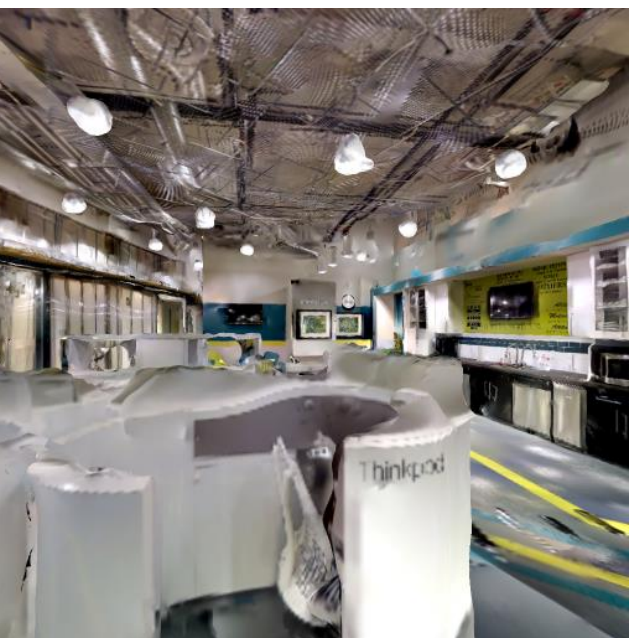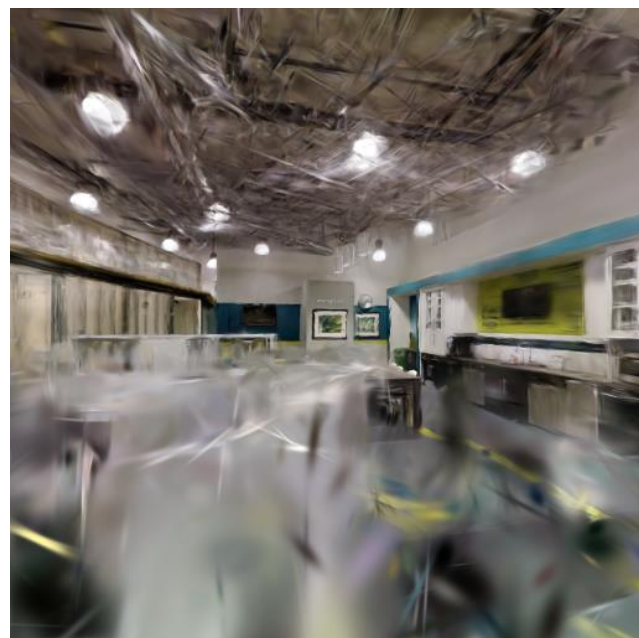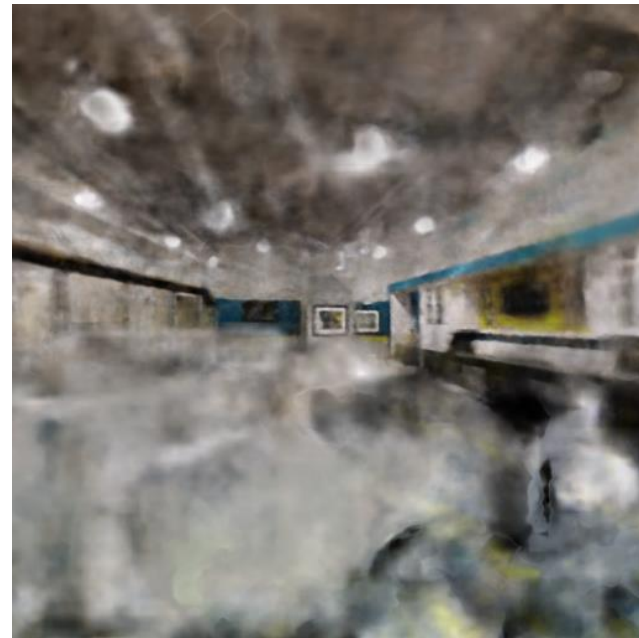

pLe4wQe7qrG

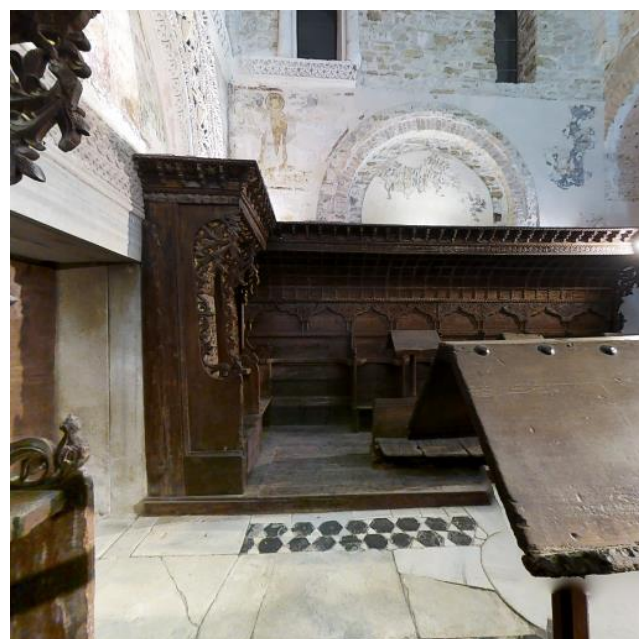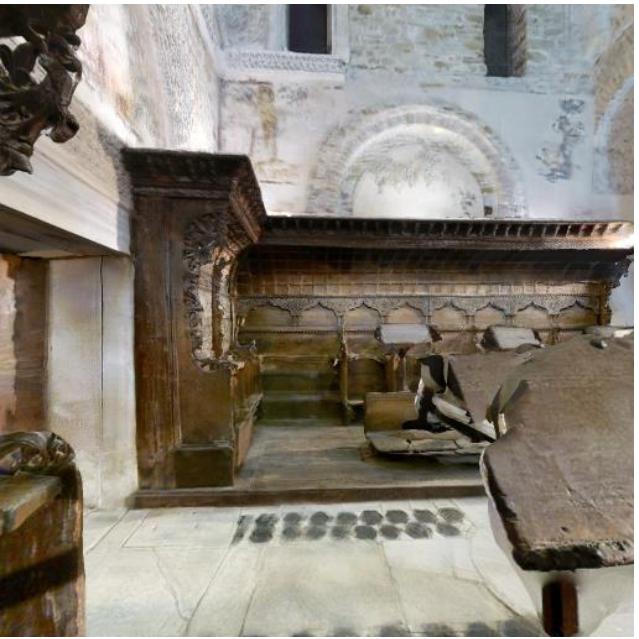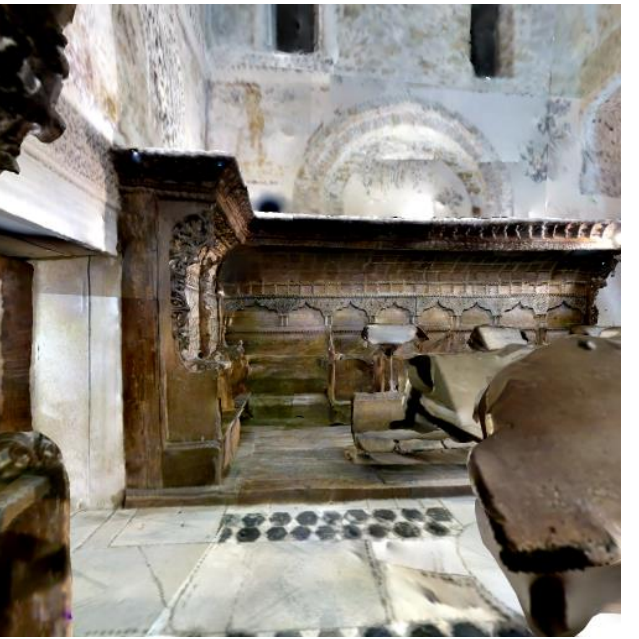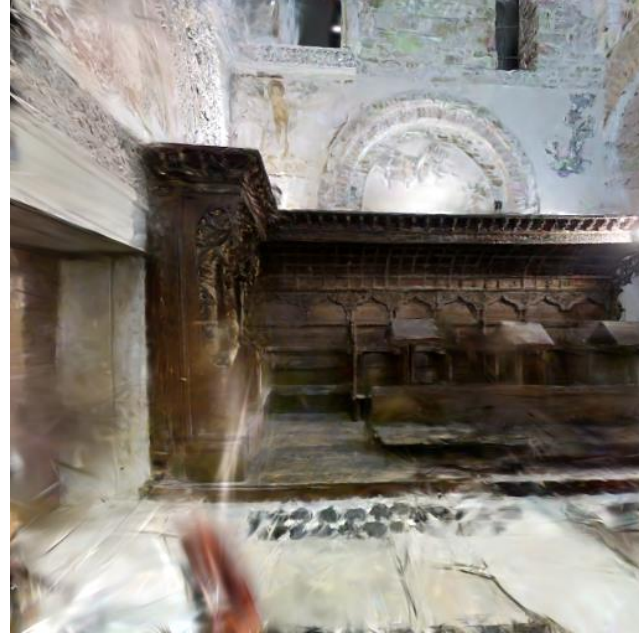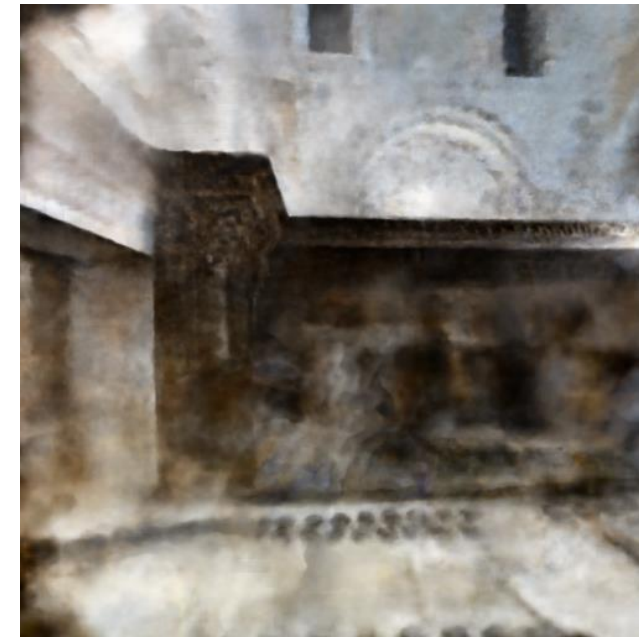

RPmz2sHmrrY

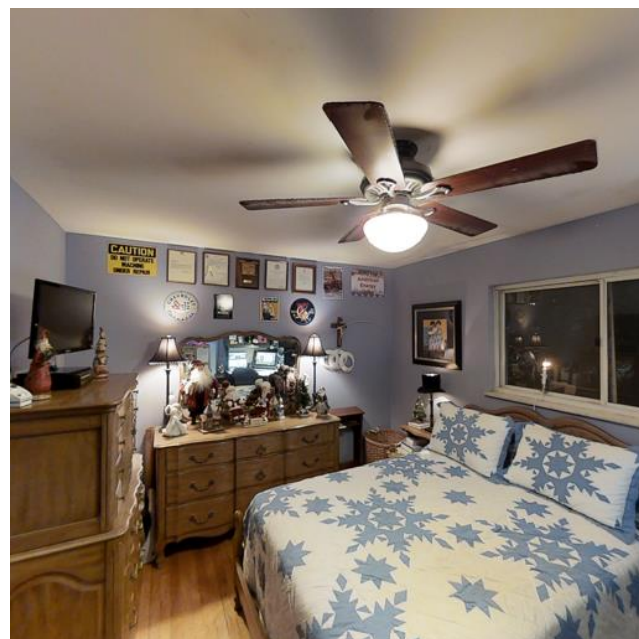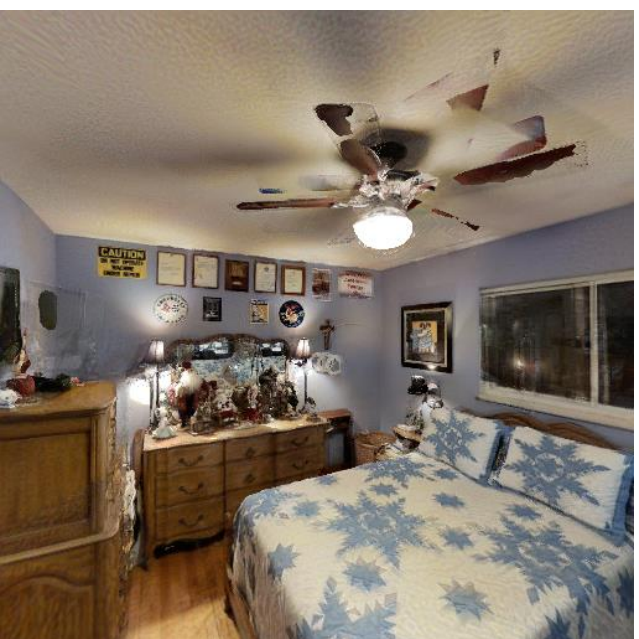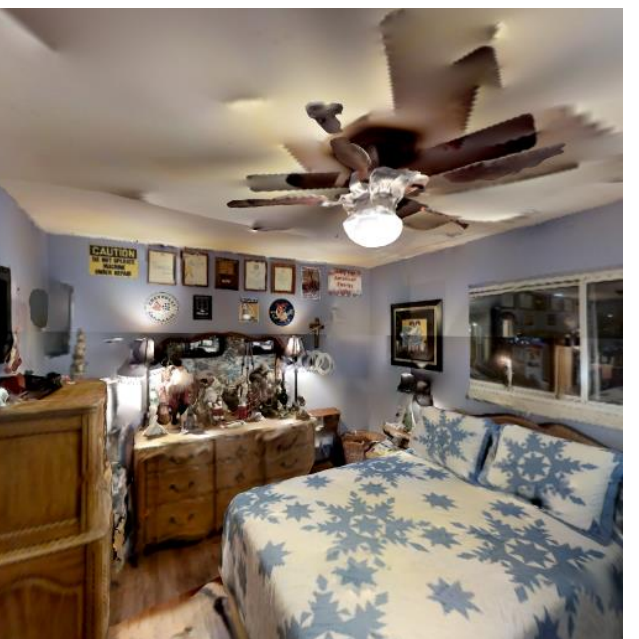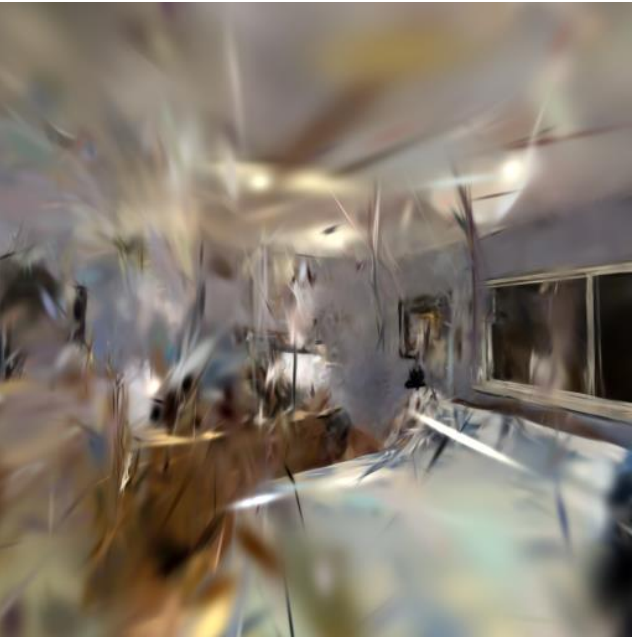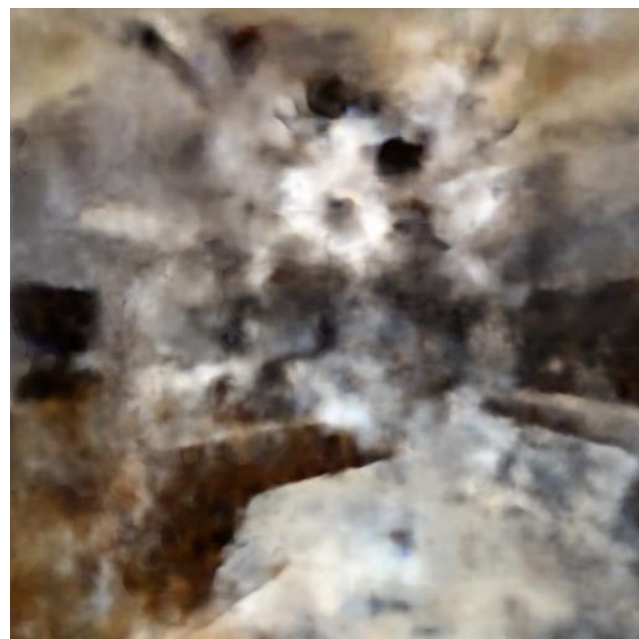

8194nk7LbLH

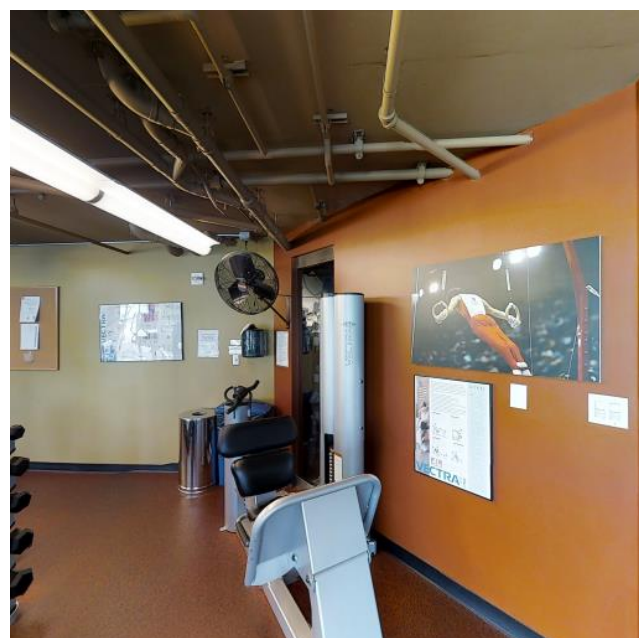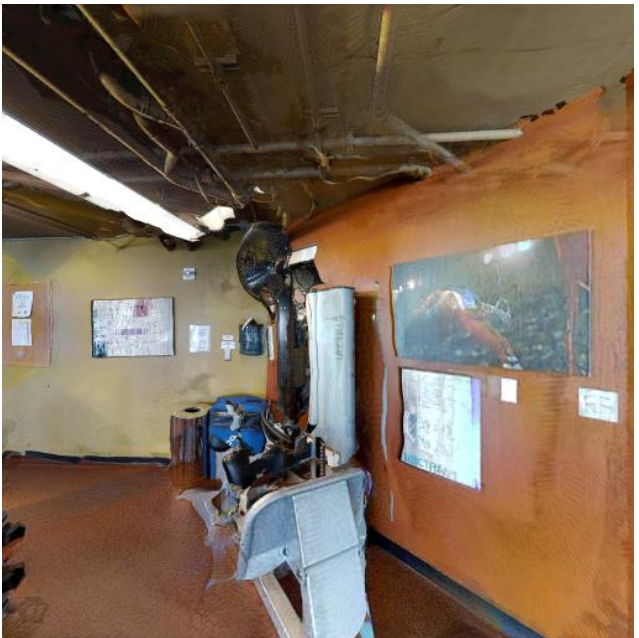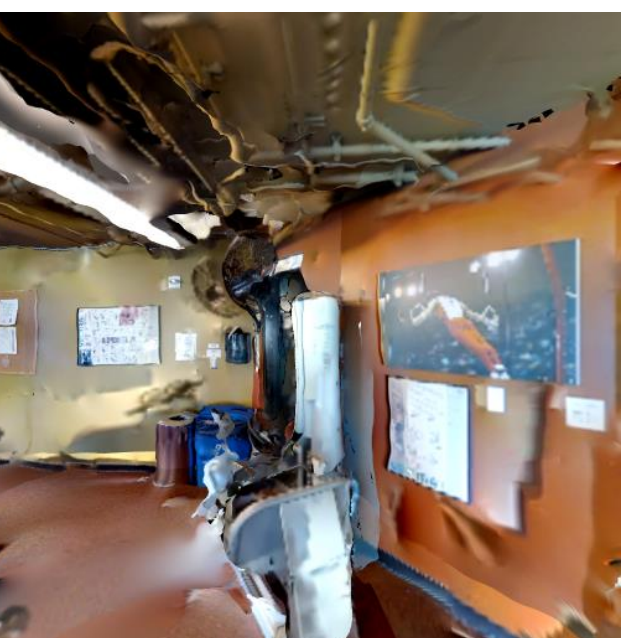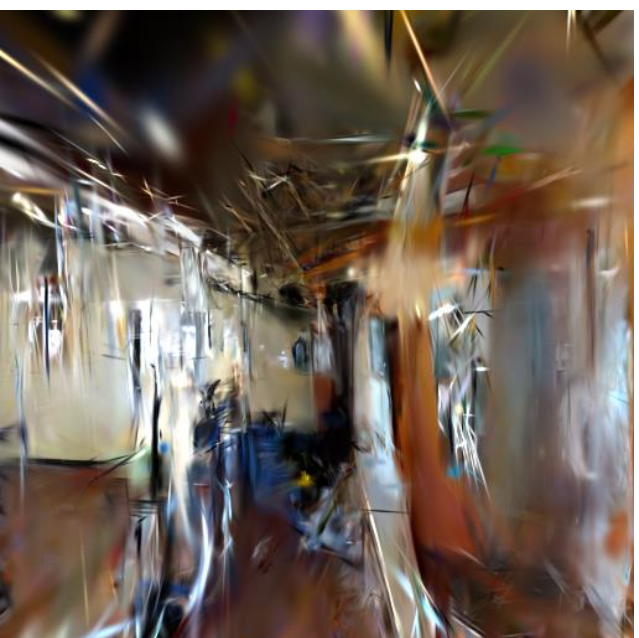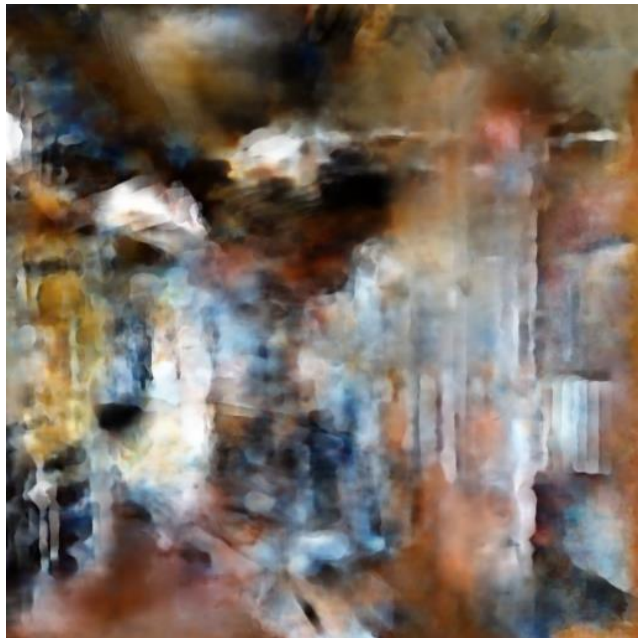

zsNo4HB9uLZ

Scene

(a) Ours

(b) TexRecon

(c) SparseGS

(d) ZipNeRF
